# Supplementary material for: Physics-guided Design and Learning of Neural Networks for Predicting Drag Force on Particle Suspensions in Moving Fluids
Source: arXiv:1911.04240 source file (2019-11-06)
Supplement: Supplementary file 1 [file appendix.tex]

\section{Dataset Description}
The dataset used has 5824 particles. Each particle has 47 input features including three-dimensional coordinates for fifteen nearest neighbors relative to the target particle's position, the Reynolds number ($Re$) and solid fraction ($\phi$) of the specific experimental setting (there are a total of 16 experimental settings with different ($Re$, $\phi$) combinations). Labels include the drag force in the X-direction $F_x \in \mathbb{R}^{1\times 1}$ as well as variables for auxiliary training, i.e., pressure fields ($\mathbf{P} \in \mathbb{R}^{10\times1}$), velocity fields ($\mathbf{V} \in \mathbb{R}^{10\times 1}$), pressure components ($\mathbf{F^P} \in \mathbb{R}^{3\times 1}$) and shear components of the drag force ($\mathbf{F^S} \in \mathbb{R}^{3\times 1}$).
\iffalse
\begin{table}[h]
\centering
\begin{tabular}{|l|l|}
\hline
 Features & Range of Data \\ \hline
$x_1, ..., x_{15}$ & $-6.75 \sim 6.71$\\
$y_1, ..., y_{15}$ & $-6.74 \sim 6.96$\\
$z_1, ..., z_{15}$ & $-7.22 \sim 7.29$\\
$Re$ & \{10, 50, 100, 200\} \\
$SF$ & \{0.1, 0.2, 0.3, 0.35\}\\\hline  
\end{tabular}
\caption{\iffalse The 47 input features of the dataset. Indexes are the column index of the features in the dataset.\fi $x_i, y_i, z_i$ corresponds to the coordinates of $i_{th}$ particle in $x, y$ and $z$ direction. The $Re$ is the Reynolds numbers. The $SF$ is global solid fractions.}
\end{table}
\fi 
\begin{table}[h]
\centering
\begin{tabular}{|l|l|}
\hline
 Features & Range of Data \\ \hline
$\mathbf{X} \in \mathbb{R}^{15\times 1}$ & $-2.93 \sim 2.95$\\
$\mathbf{Y} \in \mathbb{R}^{15\times 1}$ & $-2.96 \sim 2.95$\\
$\mathbf{Z} \in \mathbb{R}^{15\times 1}$ & $-2.96 \sim 2.96$\\
$Re \in \mathbb{R}^{1\times 1}$ & \{10, 50, 100, 200\} \\
$\phi \in \mathbb{R}^{1\times 1}$ & \{0.1, 0.2, 0.3, 0.35\}\\\hline  
\end{tabular}
\caption{The 47 input features of the dataset. Indexes are the column index of the features in the dataset. $\mathbf{X,Y,Z}$ correspond to the x, y, z coordinates respectively for the 15 nearest neighbors of a particular particle. $Re$ is the Reynolds numbers. The $\phi$ is the global solid fraction for the particular experimental setting.}
\end{table}

\begin{table}[h]
\centering
\begin{tabular}{|l|l|}
\hline
% 1. Fx-nondim
% 2 - 11. Pressure Samples 
% 12 - 21. VelocityX Samples
% 22 - 31. VelocityY Samples
% 32 - 41. VelocityZ Samples
% 42 Px
% 43 Py
% 44 Pz
% 45 TauX
% 46 TauY
% 47 TauZ
% 48 Mean Per RE,SF pair
% 49 Mask
Labels & Range of Data \\ \hline
$F_x \in \mathbb{R}^{1\times 1}$ & $0.74 \sim 107.93$\\
$\mathbf{P} \in \mathbb{R}^{10\times 1}$ & $-1.26 \sim 4.72$\\
$\mathbf{V} \in \mathbb{R}^{10\times 1}$ & $0.07 \sim 5.29$\\
$F^P_x \in \mathbb{R}^{1\times 1}$ & $0.27 \sim 92.32$ \\
$F^P_y \in \mathbb{R}^{1\times 1}$ & $-15.54 \sim 19.61$ \\
$F^P_z \in \mathbb{R}^{1\times 1}$ & $-14.23 \sim 15.28$ \\
$F^S_x \in \mathbb{R}^{1\times 1}$ & $0.42 \sim 17.19$ \\
$F^S_y \in \mathbb{R}^{1\times 1}$ & $-2.88 \sim 3.57$\\
$F^S_z \in \mathbb{R}^{1\times 1}$ & $-2.95 \sim 5.05$\\
\hline  
\end{tabular}
\caption{\iffalse The 47 labels of the dataset. Indexes are the column index of the labels in the dataset.\fi $F_x$ is the drag force the particle experienced on the $x$ direction, which is the target variable to predict. $F^P_x,F^P_y,F^P_z$ represent the pressure drag components in the x,y,z directions respectively. $F^S_x,F^S_y,F^S_z$ represent the shear drag components in the x,y,z directions respectively.}
\end{table}

\iffalse 
\begin{table}[h]
\centering
\begin{tabular}{|l|l|}
\hline
% 1. Fx-nondim
% 2 - 11. Pressure Samples 
% 12 - 21. VelocityX Samples
% 22 - 31. VelocityY Samples
% 32 - 41. VelocityZ Samples
% 42 Px
% 43 Py
% 44 Pz
% 45 TauX
% 46 TauY
% 47 TauZ
% 48 Mean Per RE,SF pair
% 49 Mask
Labels & Range of Data \\ \hline
$F_x$ & $0.74 \sim 107.93$\\
$p_1, ..., p_{10}$ & $-1.26 \sim 4.72$\\
$v_{x1}, ..., v_{x10}$ & $0.07 \sim 5.29$\\
$v_{y1}, ..., v_{y10}$ & $-0.57 \sim 0.62$\\
$v_{z1}, ..., v_{z10}$ & $-0.48 \sim 0.63$\\
$P_x$ & $-7.22 \sim 7.29$ \\
$P_y$ & $-7.22 \sim 7.29$ \\
$P_z$ & $-7.22 \sim 7.29$ \\
$Tau_x$ & $-7.22 \sim 7.29$ \\
$Tau_y$ & $0.056 \sim 0.528$\\
$Tau_z$ & $0.056 \sim 0.528$\\
\hline  
\end{tabular}
\caption{\iffalse The 47 labels of the dataset. Indexes are the column index of the labels in the dataset.\fi $F_x$ is the drag force the particle experienced on the $x$ direction, which is the objective variable to predict. $p_j, v_{xj}, v_{yj}, v_{zj}$ are the pressure field values, velocity field values in $x, y$ and $z$ directions on the 10 sampling points around a particle.}
\end{table}
\fi 
\section{Experimental Results}
\subsection{Characterizing \ourmethodAll Performance For Different (Re,$\,\phi$) Settings.}
\iffalse Thus far, we have reported performance results of our \ourmethodAll model qunatitatively for the 0.55 training fraction. However, these results are a combination of predictions made over different (Re,$\phi$) settings.\fi  In addition to quantitative evaluation, qualitative inspection is necessary for a deeper, holistic understanding of model behavior. Hence, we showcase the particle drag force predictions by the \ourmethodAll model for different (Re,$\phi$) combinations in Fig.~\ref{fig:prs_scatter_plots}. We notice that the \ourmethodAll model yields accurate predictions (i.e yellow and red curves are aligned). This indicates that the \ourmethodAll model is able to effectively capture sophisticated particle interactions and the consequent effect of said interactions on the drag forces of the interacting particles. \iffalse The increase in problem complexity with increase in solid fraction is apparent in Fig.~\ref{fig:re_10_sf_20} - Fig.~\ref{fig:re_10_sf_35}, where we notice that the yellow curve representing the ground truth particle drag force data, transitions from a near linear representation in Fig.~\ref{fig:re_10_sf_20} (Re=10,$\phi$=0.2) to a significantly more nonlinear representation in Fig.~\ref{fig:re_10_sf_35} (Re=10,$\phi$=0.35).\fi  We notice that for high (Re,$\phi$) as in Fig.~\ref{fig:re_200_sf_35}, the drag force i.e PRS curve (yellow) is nonlinear in nature and that the magnitude of drag forces is also higher at higher (Re,$\phi$) settings. Such differing scales of drag force values can also complicate the drag force prediction problem as it is non-trivial for a single model to effectively learn such multi-modal target distributions. However, we find that the \ourmethodAll model is effective in this setting.  
\begin{figure*}[!htpb]
     \centering
     \begin{subfigure}[b]{0.48\columnwidth}
         \centering
         \includegraphics[width=\textwidth]{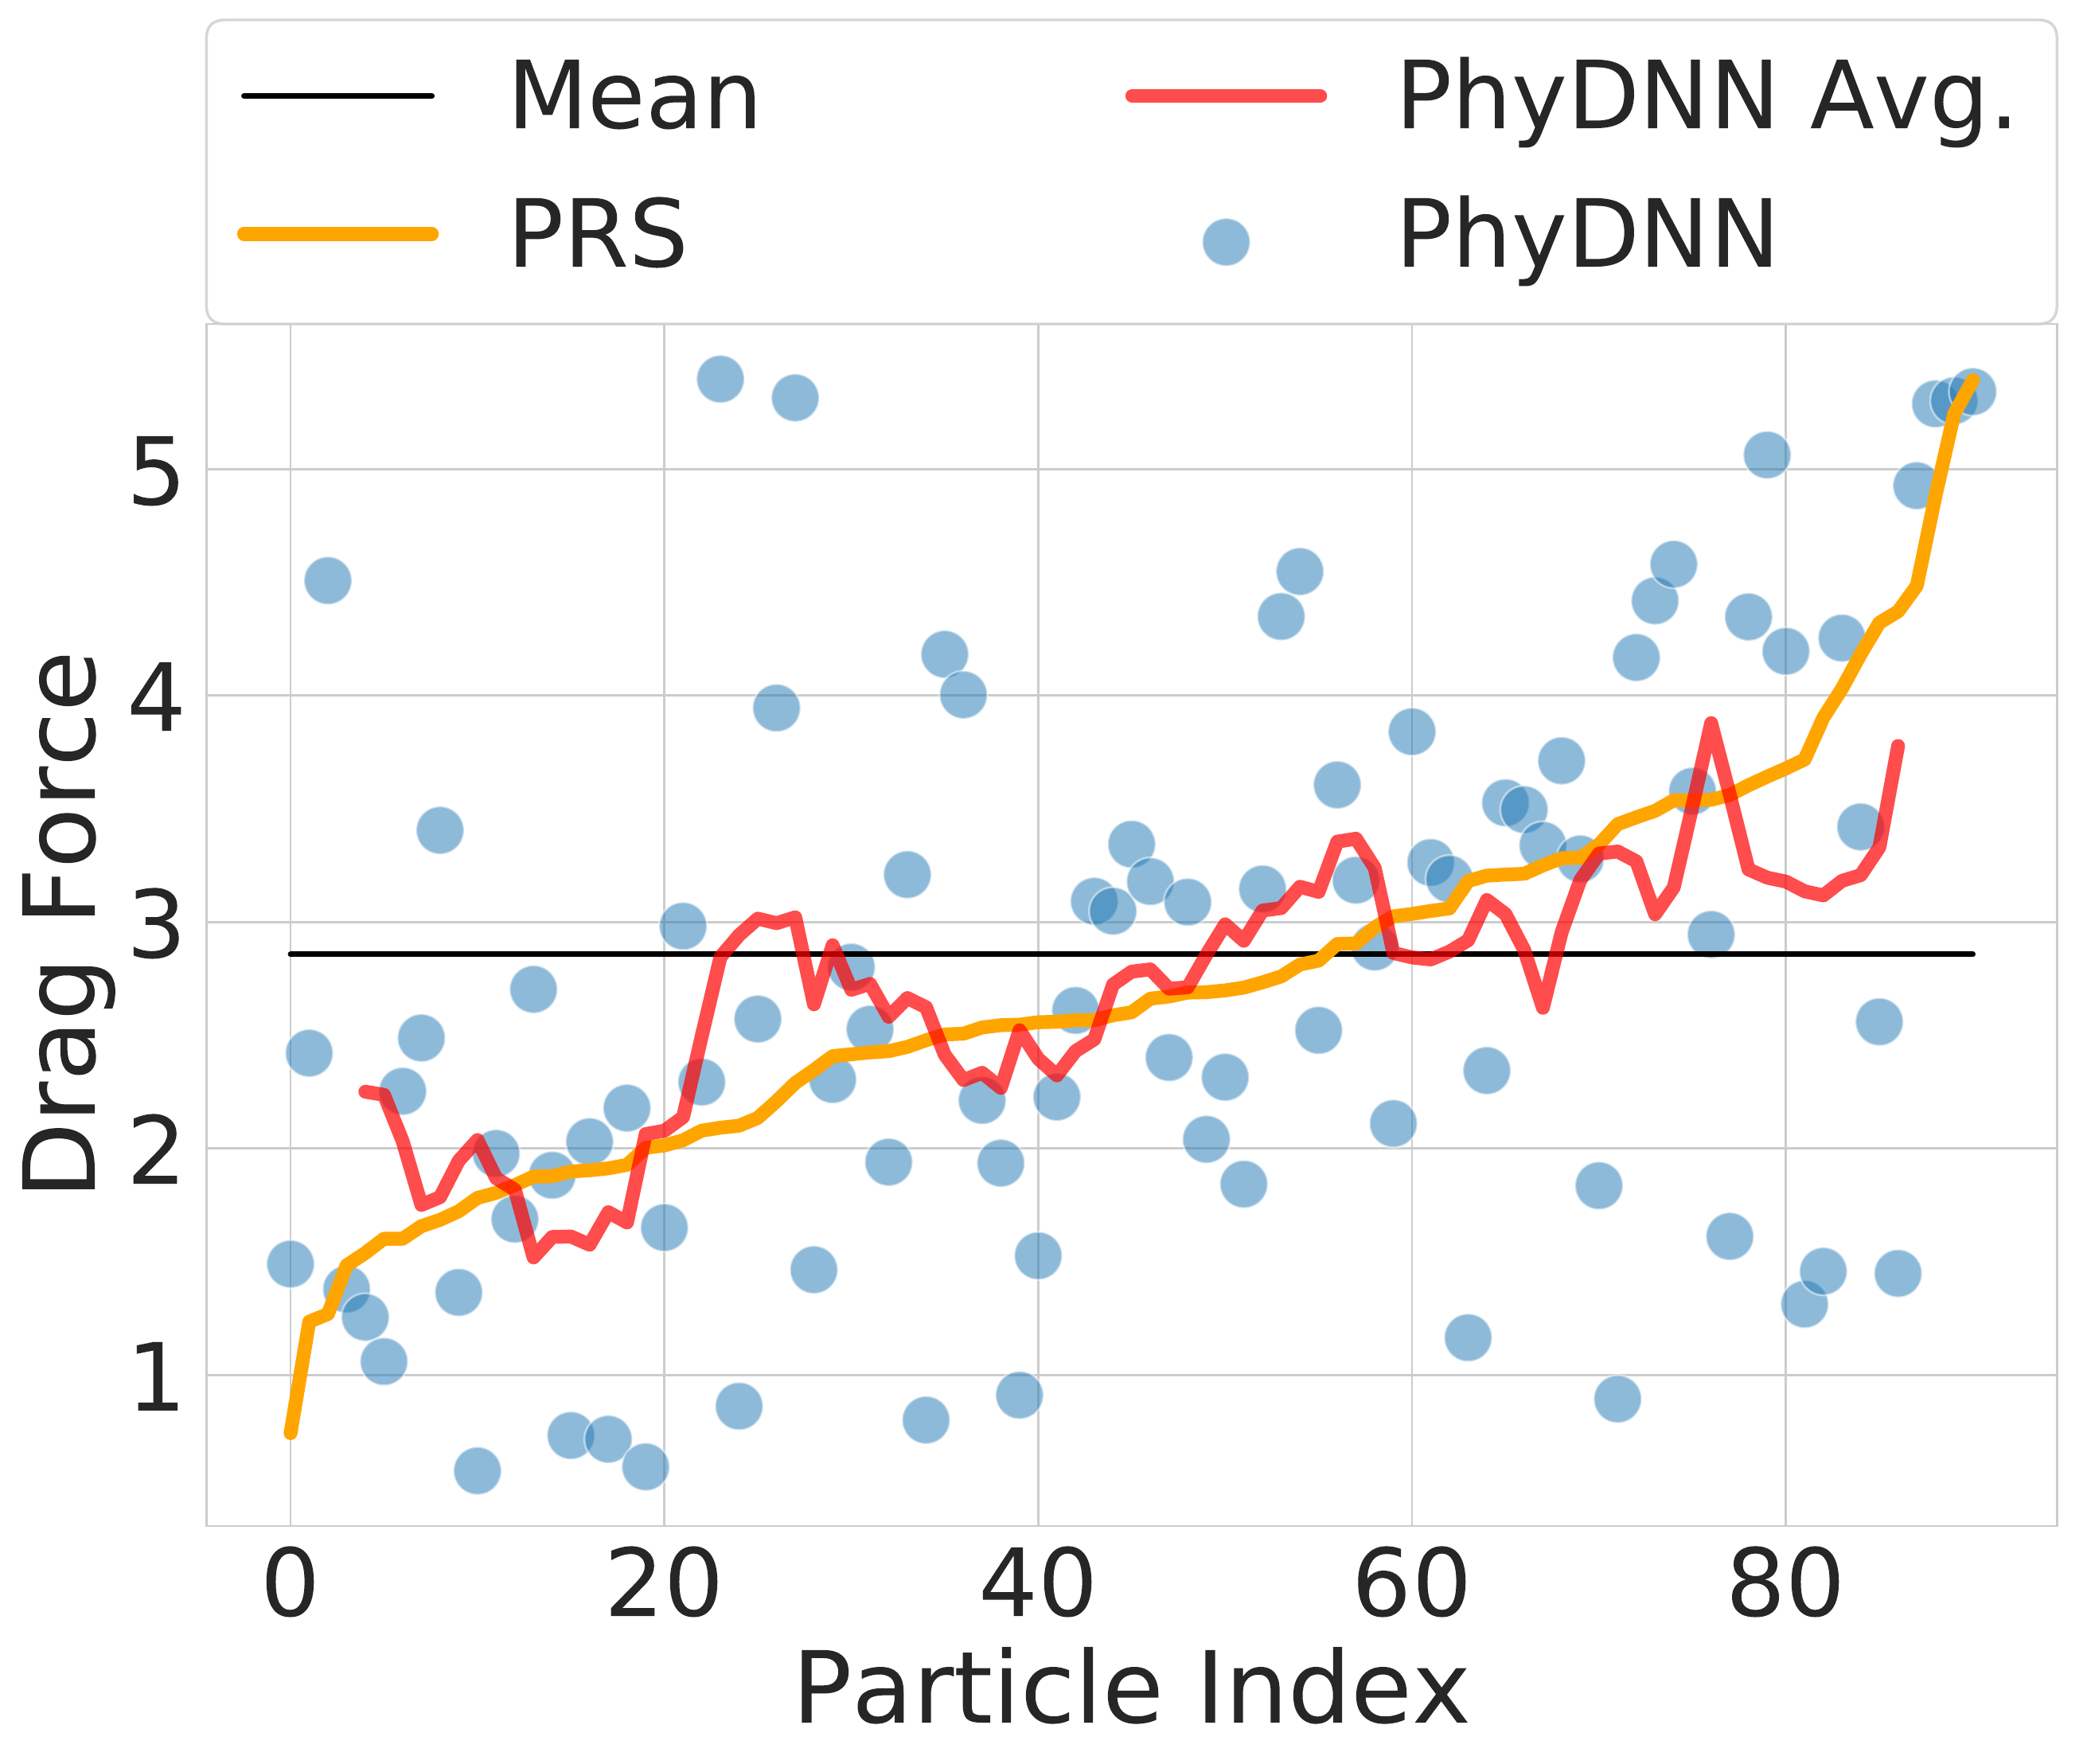}
         \caption{$Re=10,\phi = 0.1$}
         \label{fig:re_10_sf_10}
     \end{subfigure}
     \hfill
     \begin{subfigure}[b]{0.48\columnwidth}
         \includegraphics[width=\textwidth]{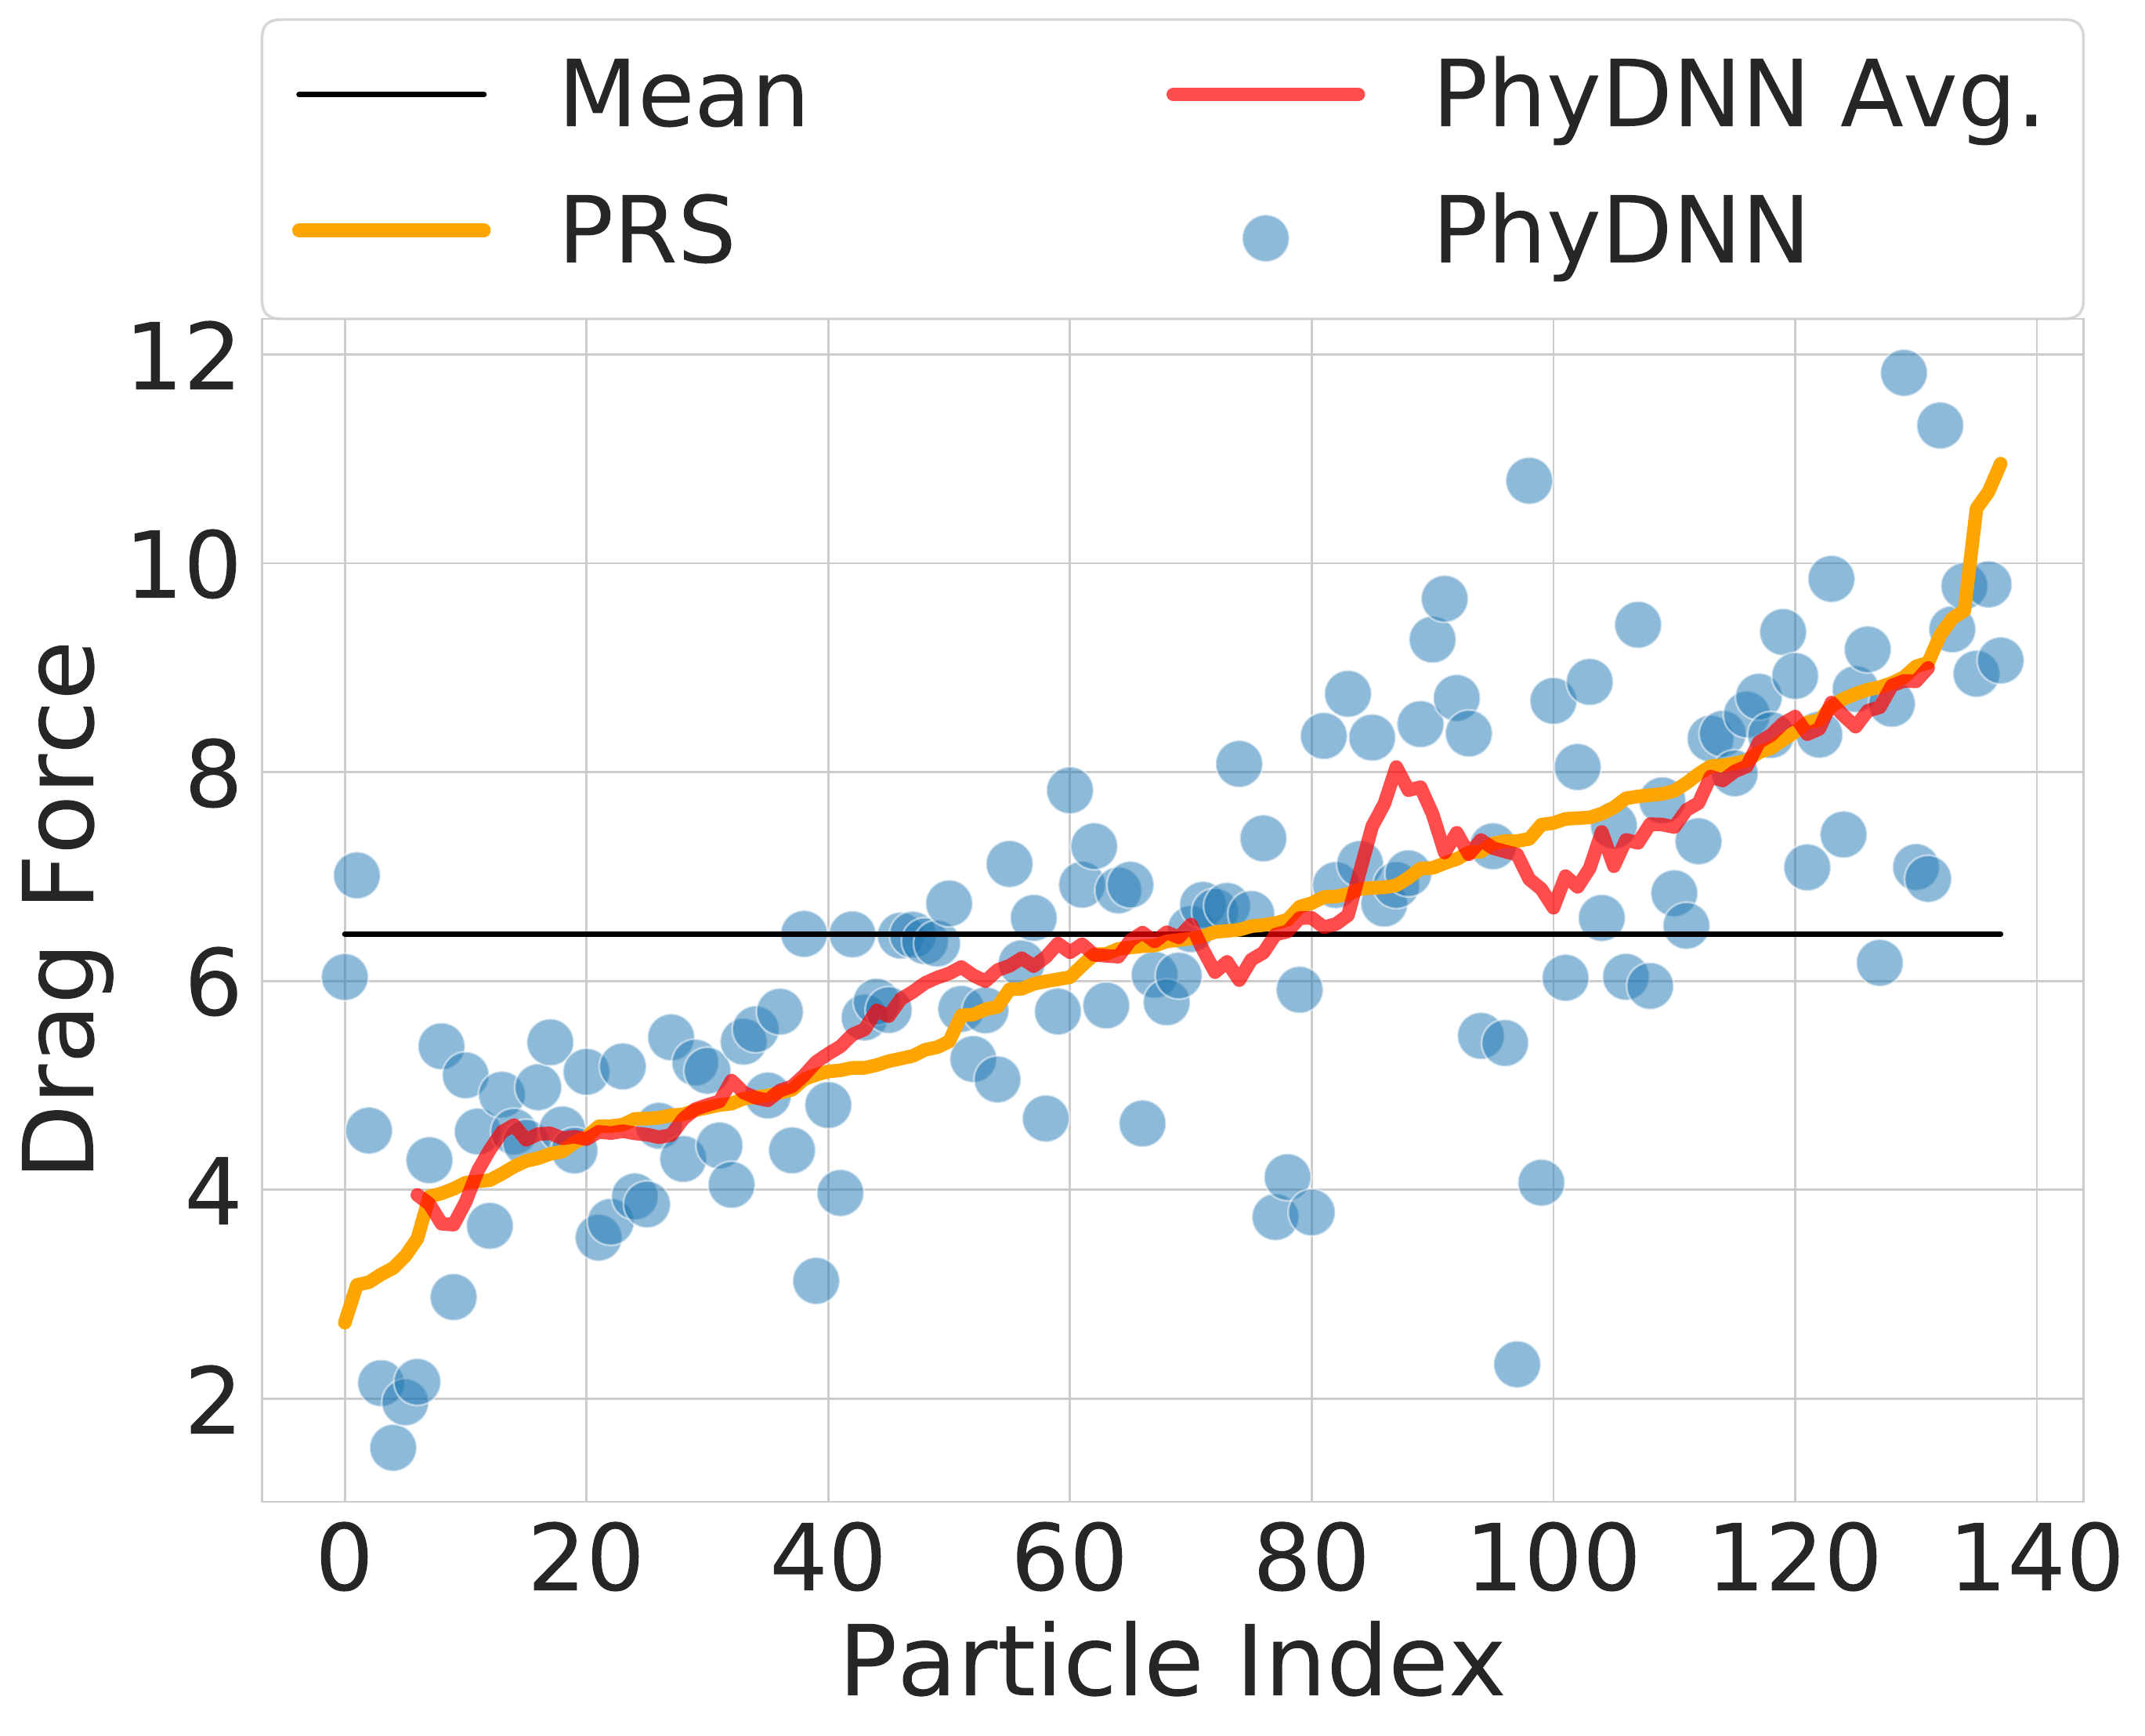}
         \caption{$Re = 10, \phi = 0.2$}
         \label{fig:re_10_sf_20}
     \end{subfigure}
     \hfill
     \begin{subfigure}[b]{0.48\columnwidth}         \includegraphics[width=\textwidth]{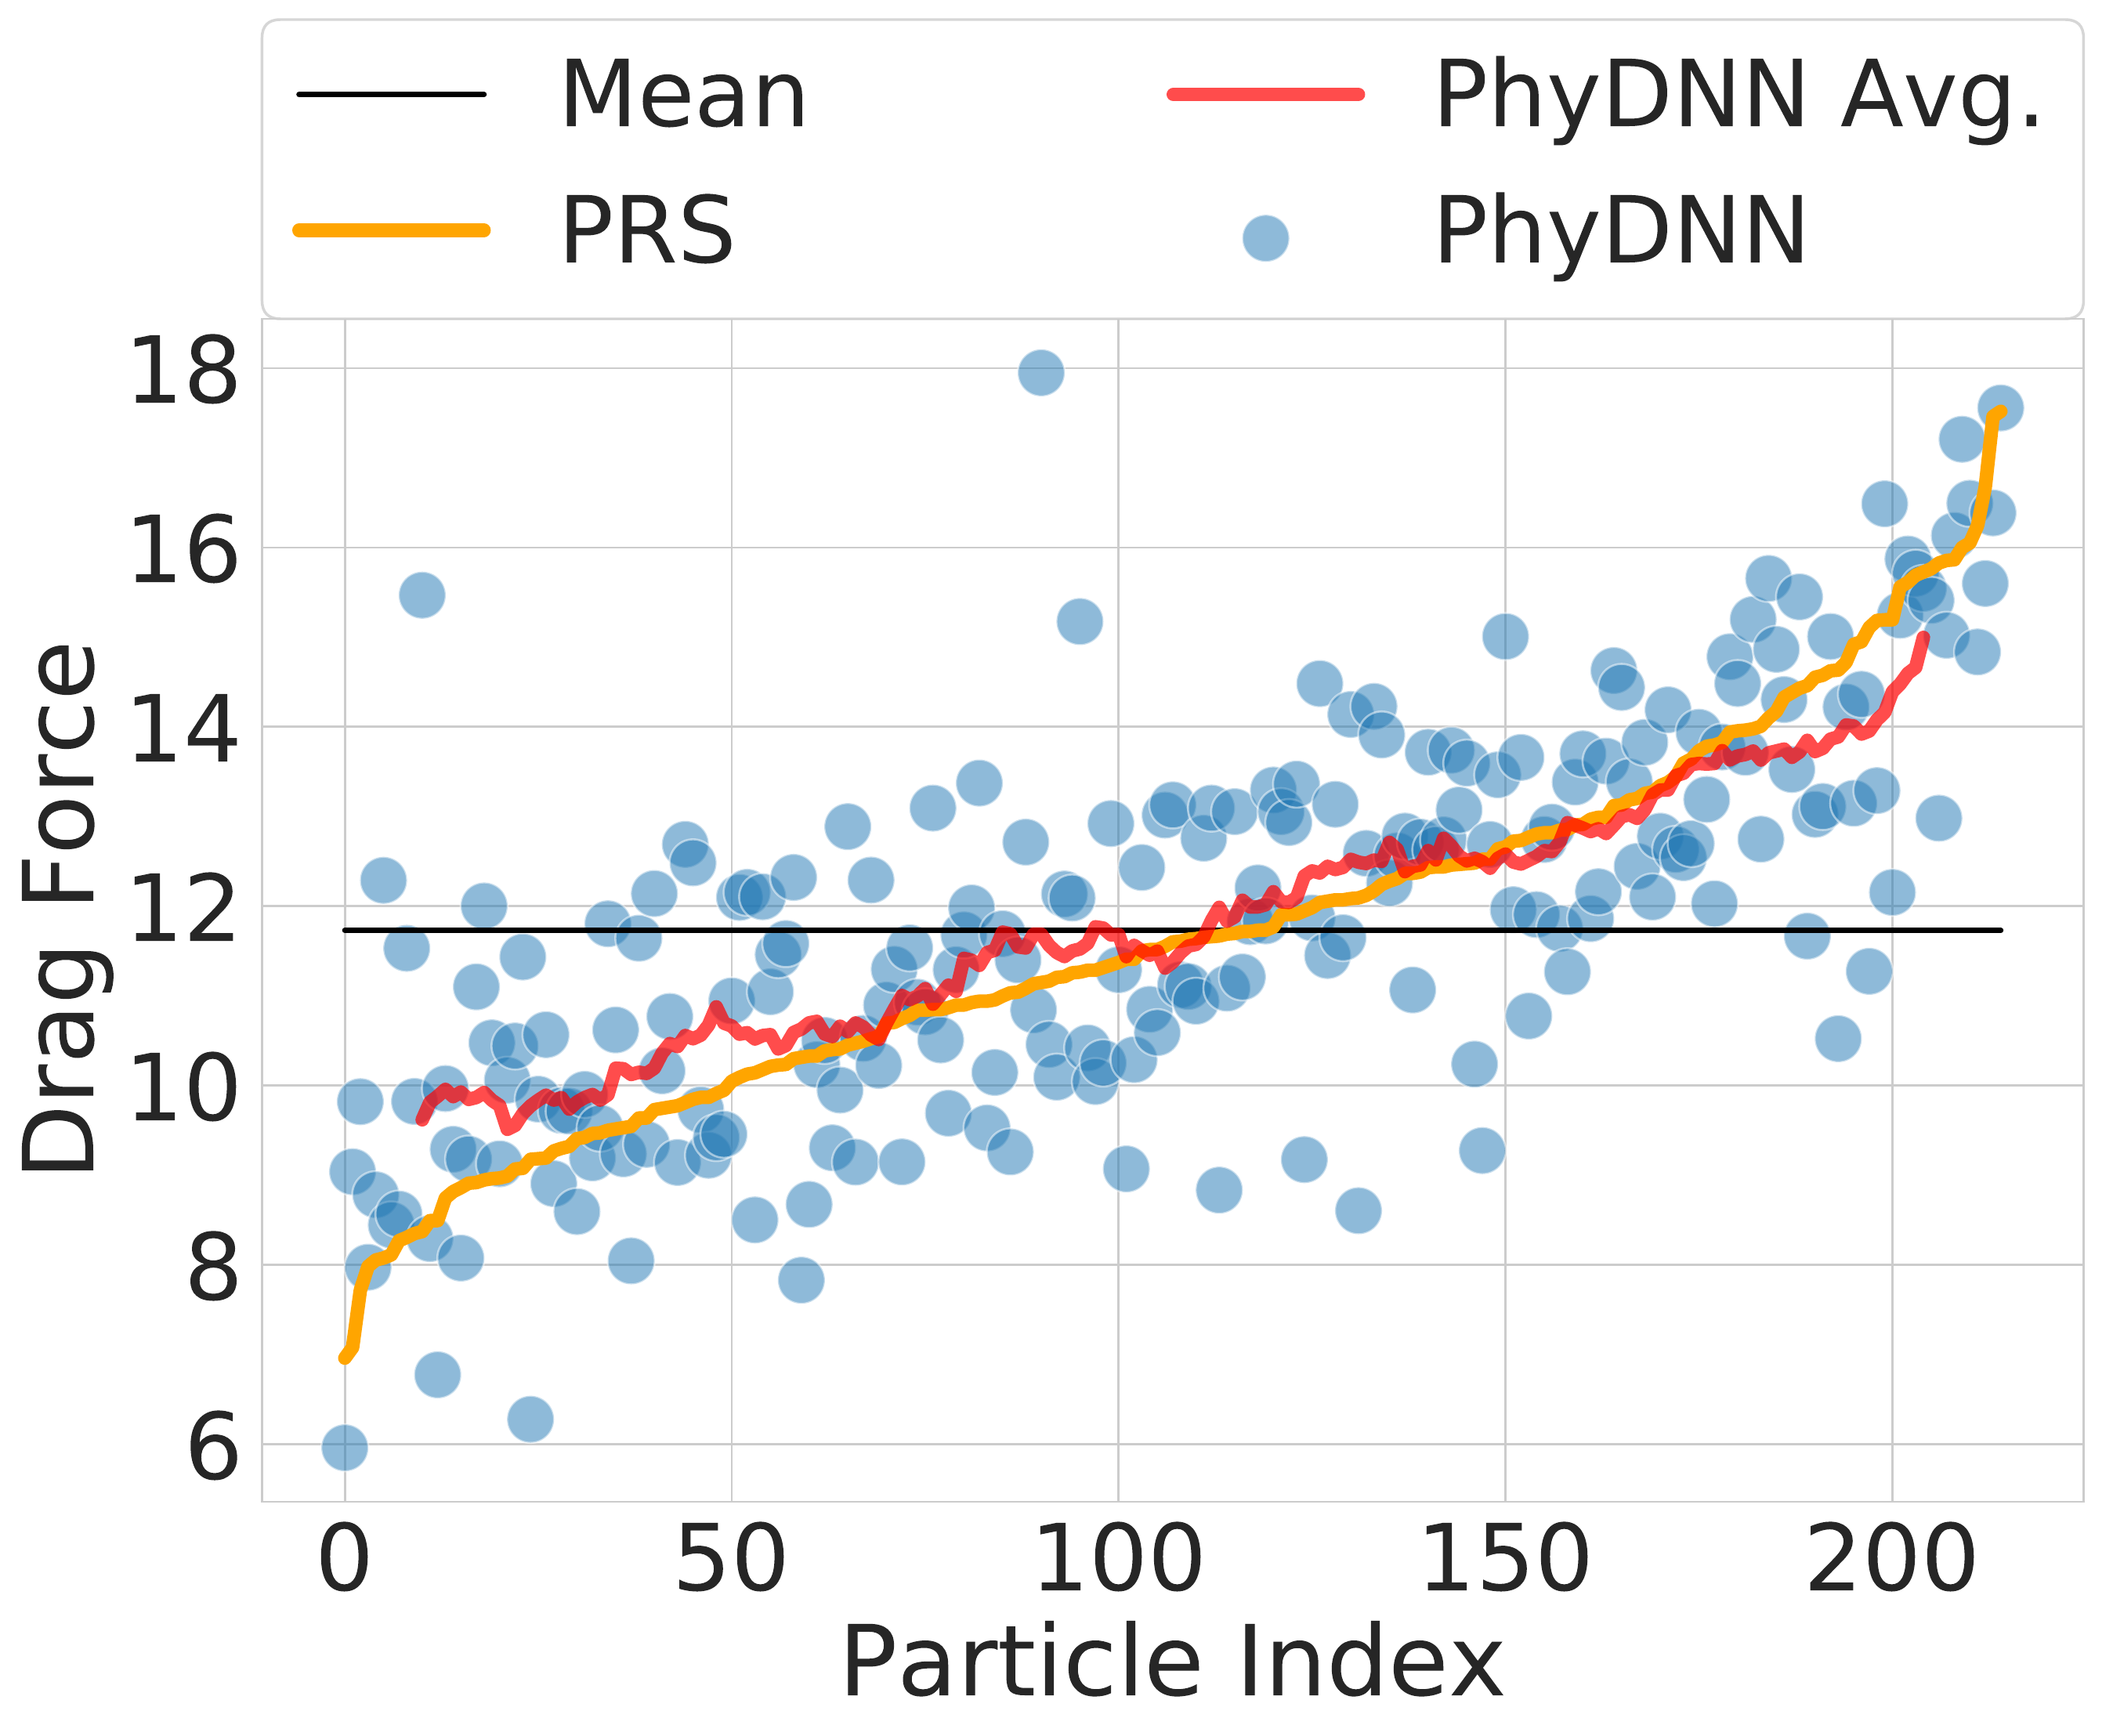}
         \caption{$Re = 10, \phi = 0.3$}
         \label{fig:re_10_sf_30}
     \end{subfigure}
     \hfill
     \begin{subfigure}[b]{0.48\columnwidth}
         \centering
         \includegraphics[width=\textwidth]{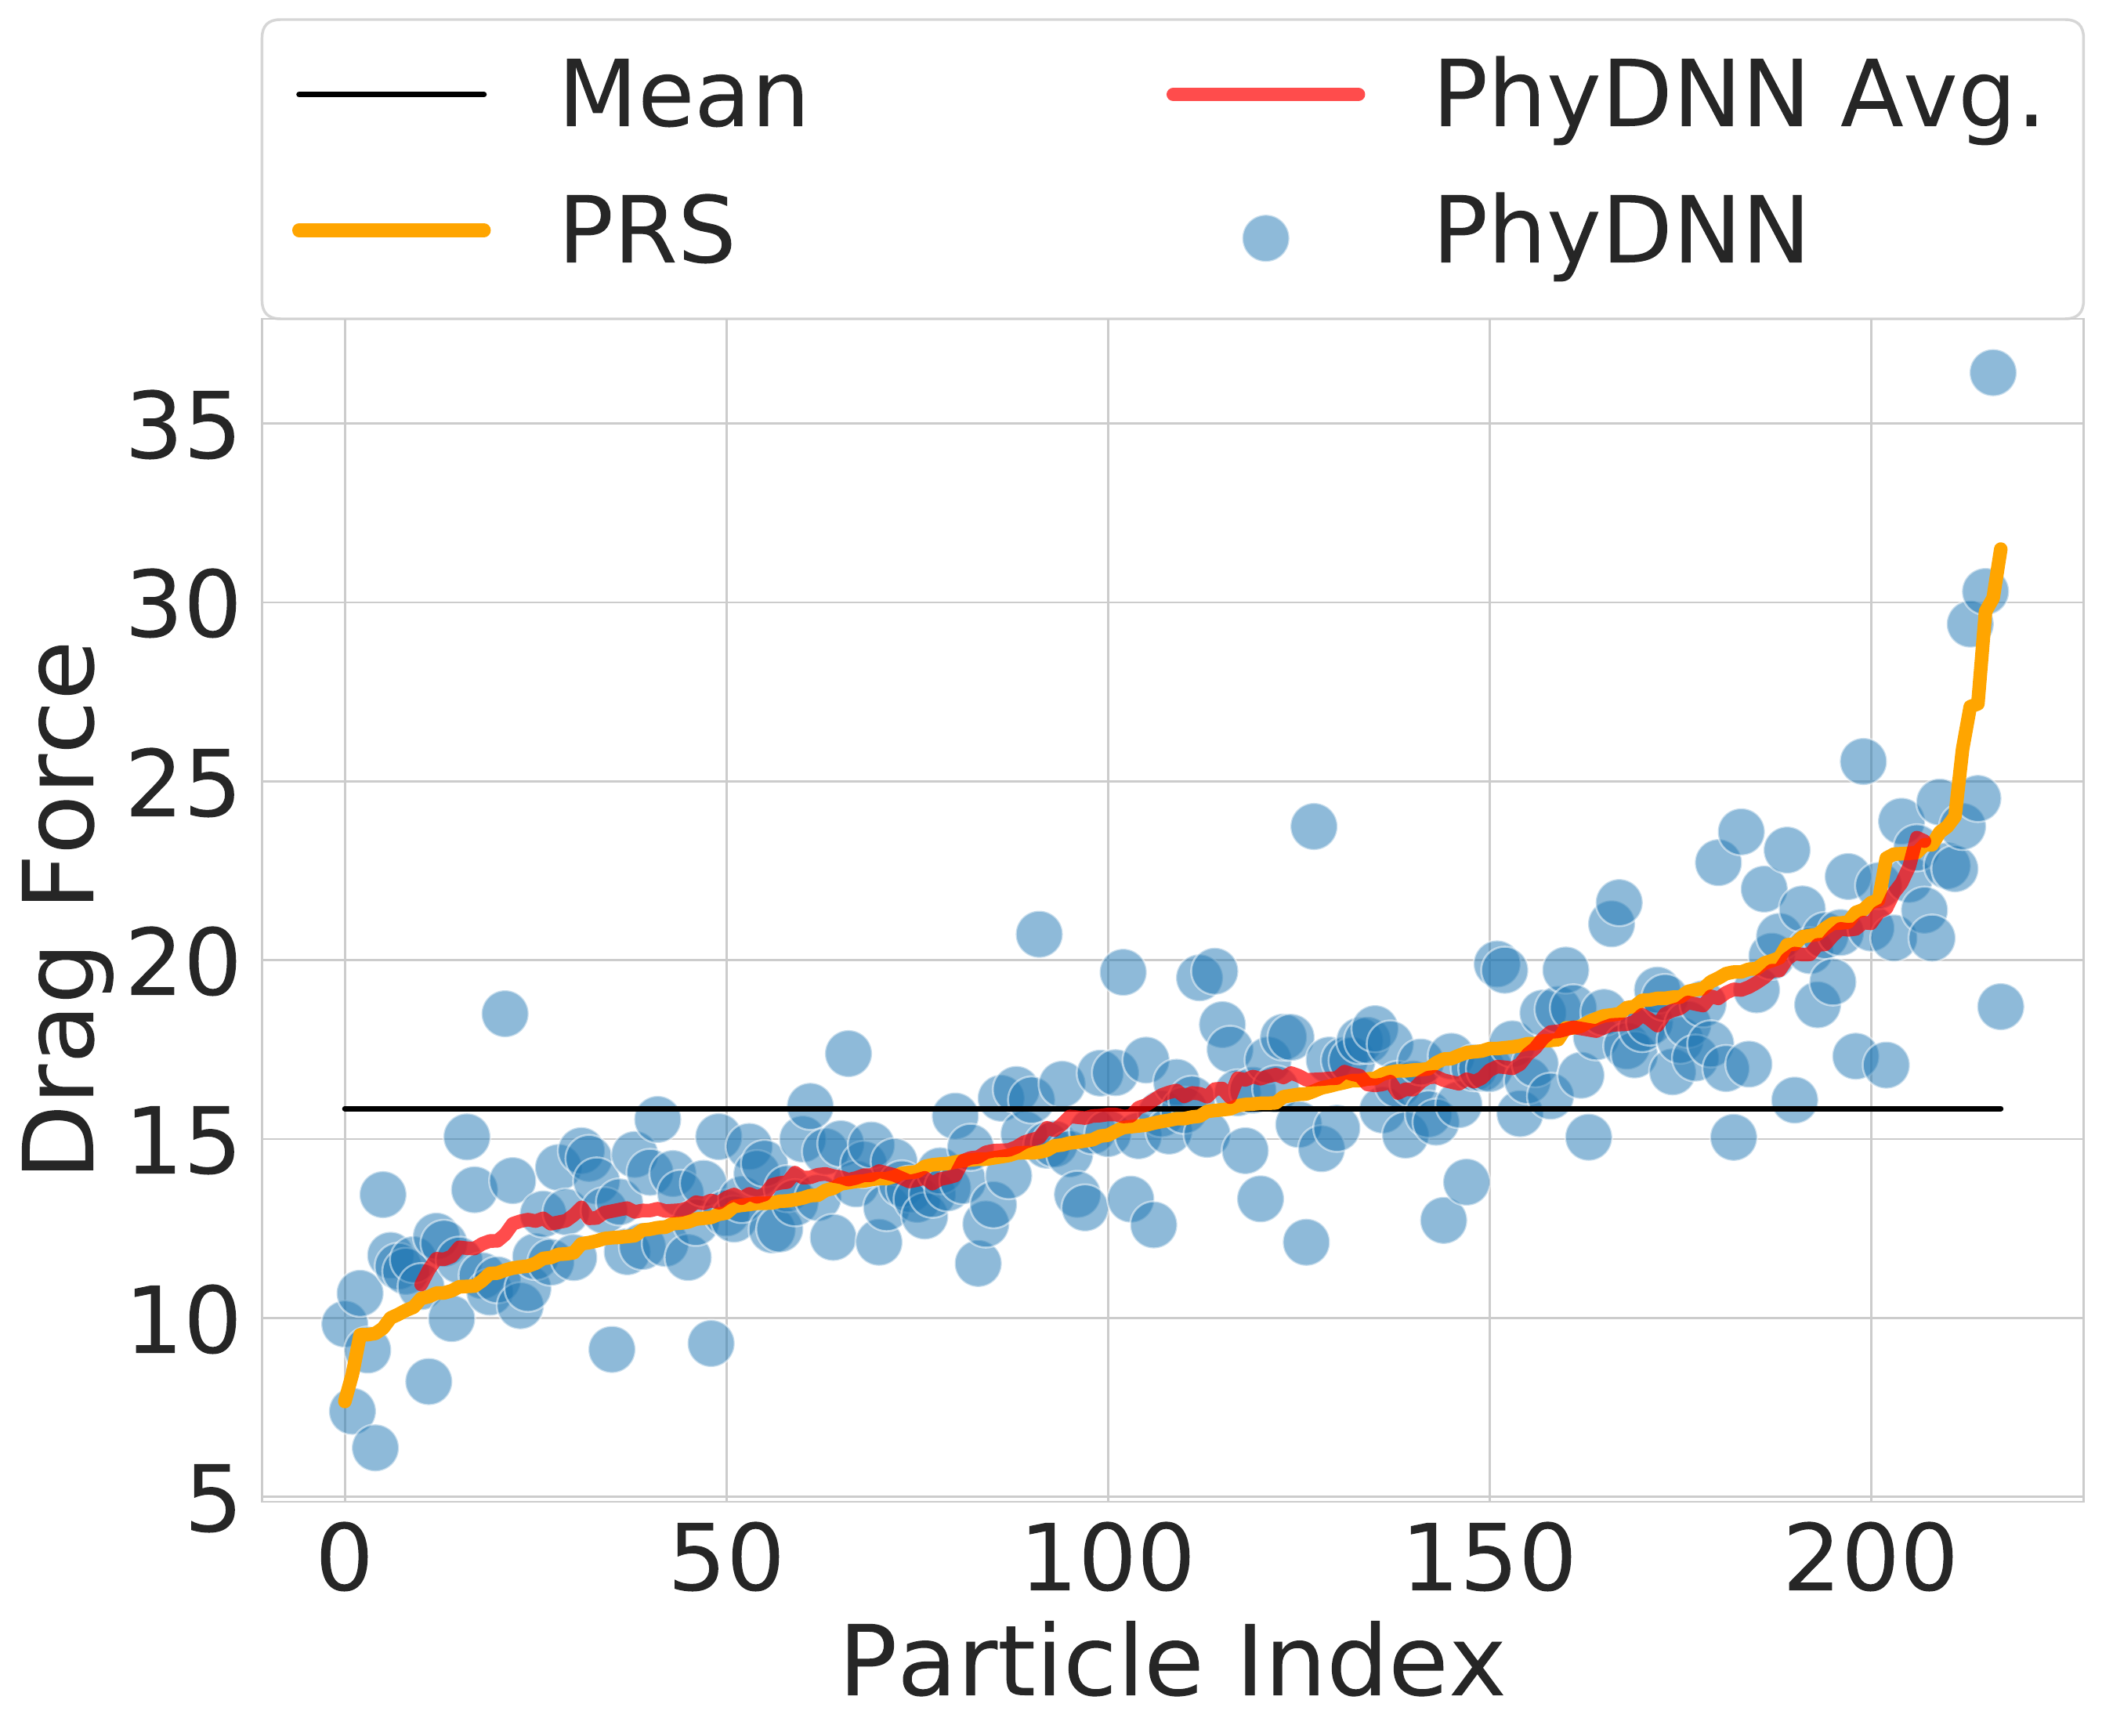}
         \caption{$Re = 10, \phi = 0.35$}
         \label{fig:re_10_sf_35}
     \end{subfigure}
     \vfill  %%%%%%%%%%%%%%%%%%%%%%%%%%%%%%%%%%%%%%%%%%%%%%%%%%%%%%%%%%%%%%%%%%%%%%%%%%%%%%%%%%%%%%%%%%%%
     \begin{subfigure}[b]{0.48\columnwidth}         \includegraphics[width=\textwidth]{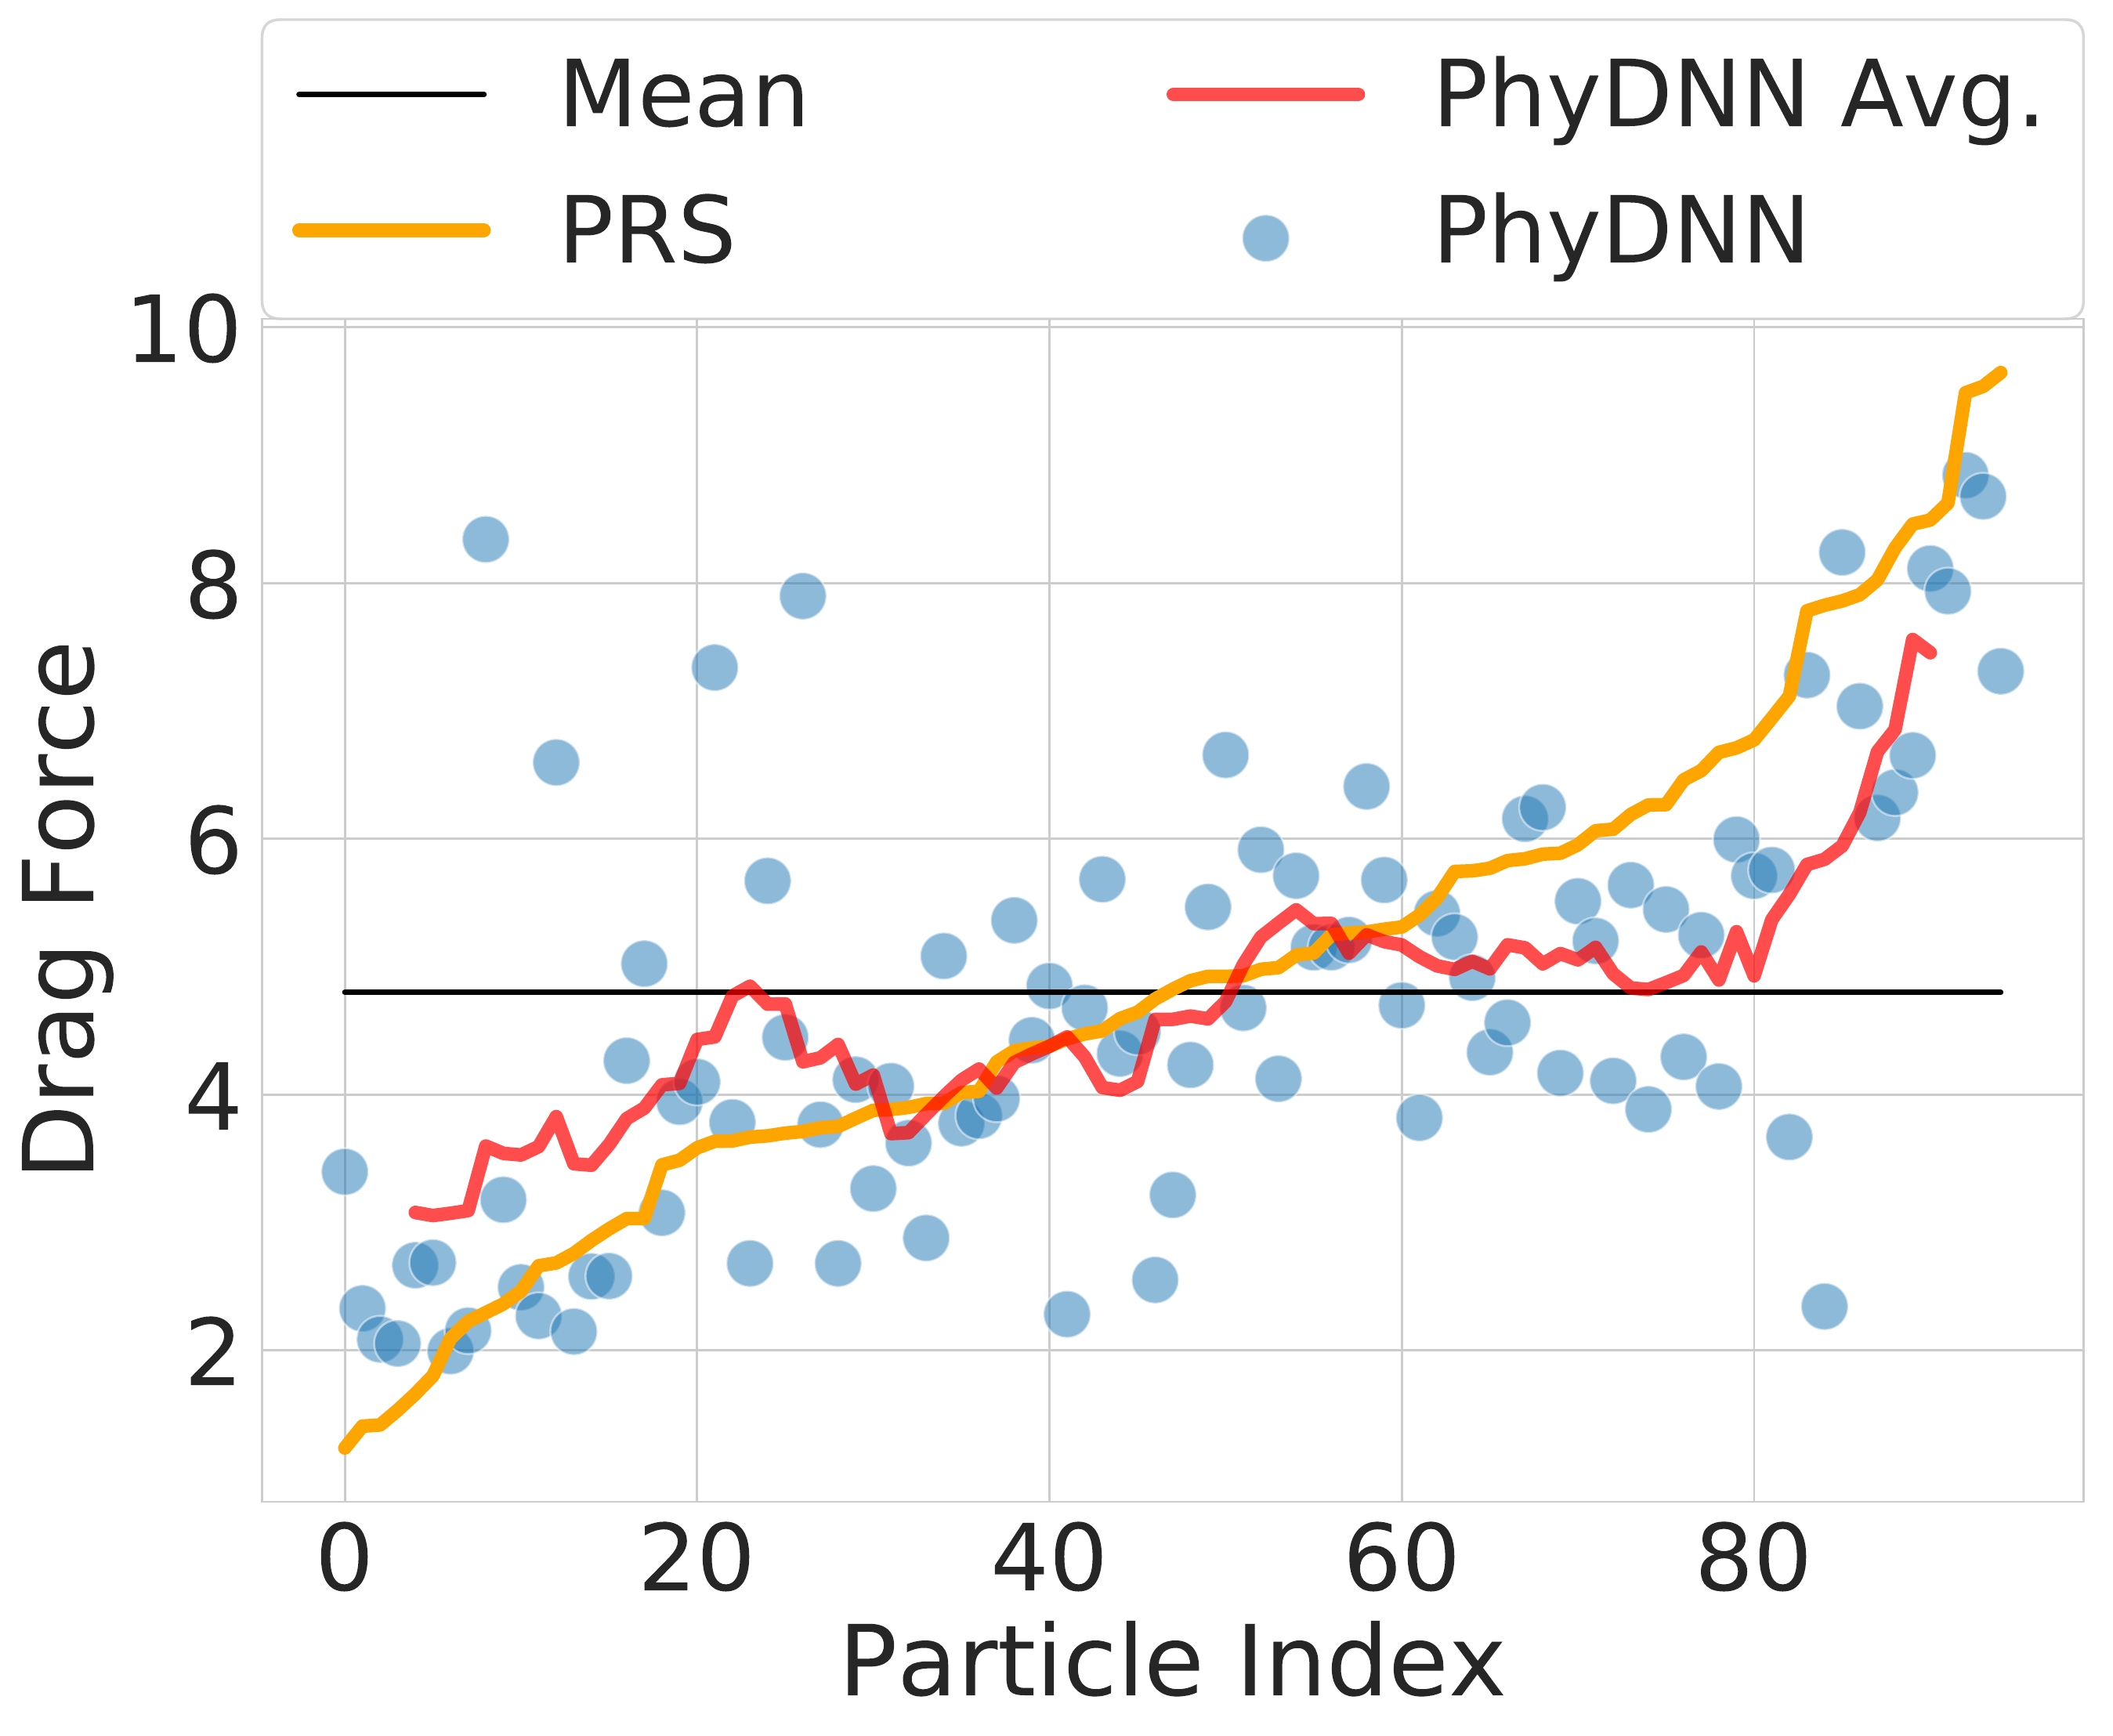}
         \caption{$Re = 50, \phi = 0.1$}
         \label{fig:re_50_sf_10}
     \end{subfigure}
     \hfill
     \begin{subfigure}[b]{0.48\columnwidth}
         \centering
         \includegraphics[width=\textwidth]{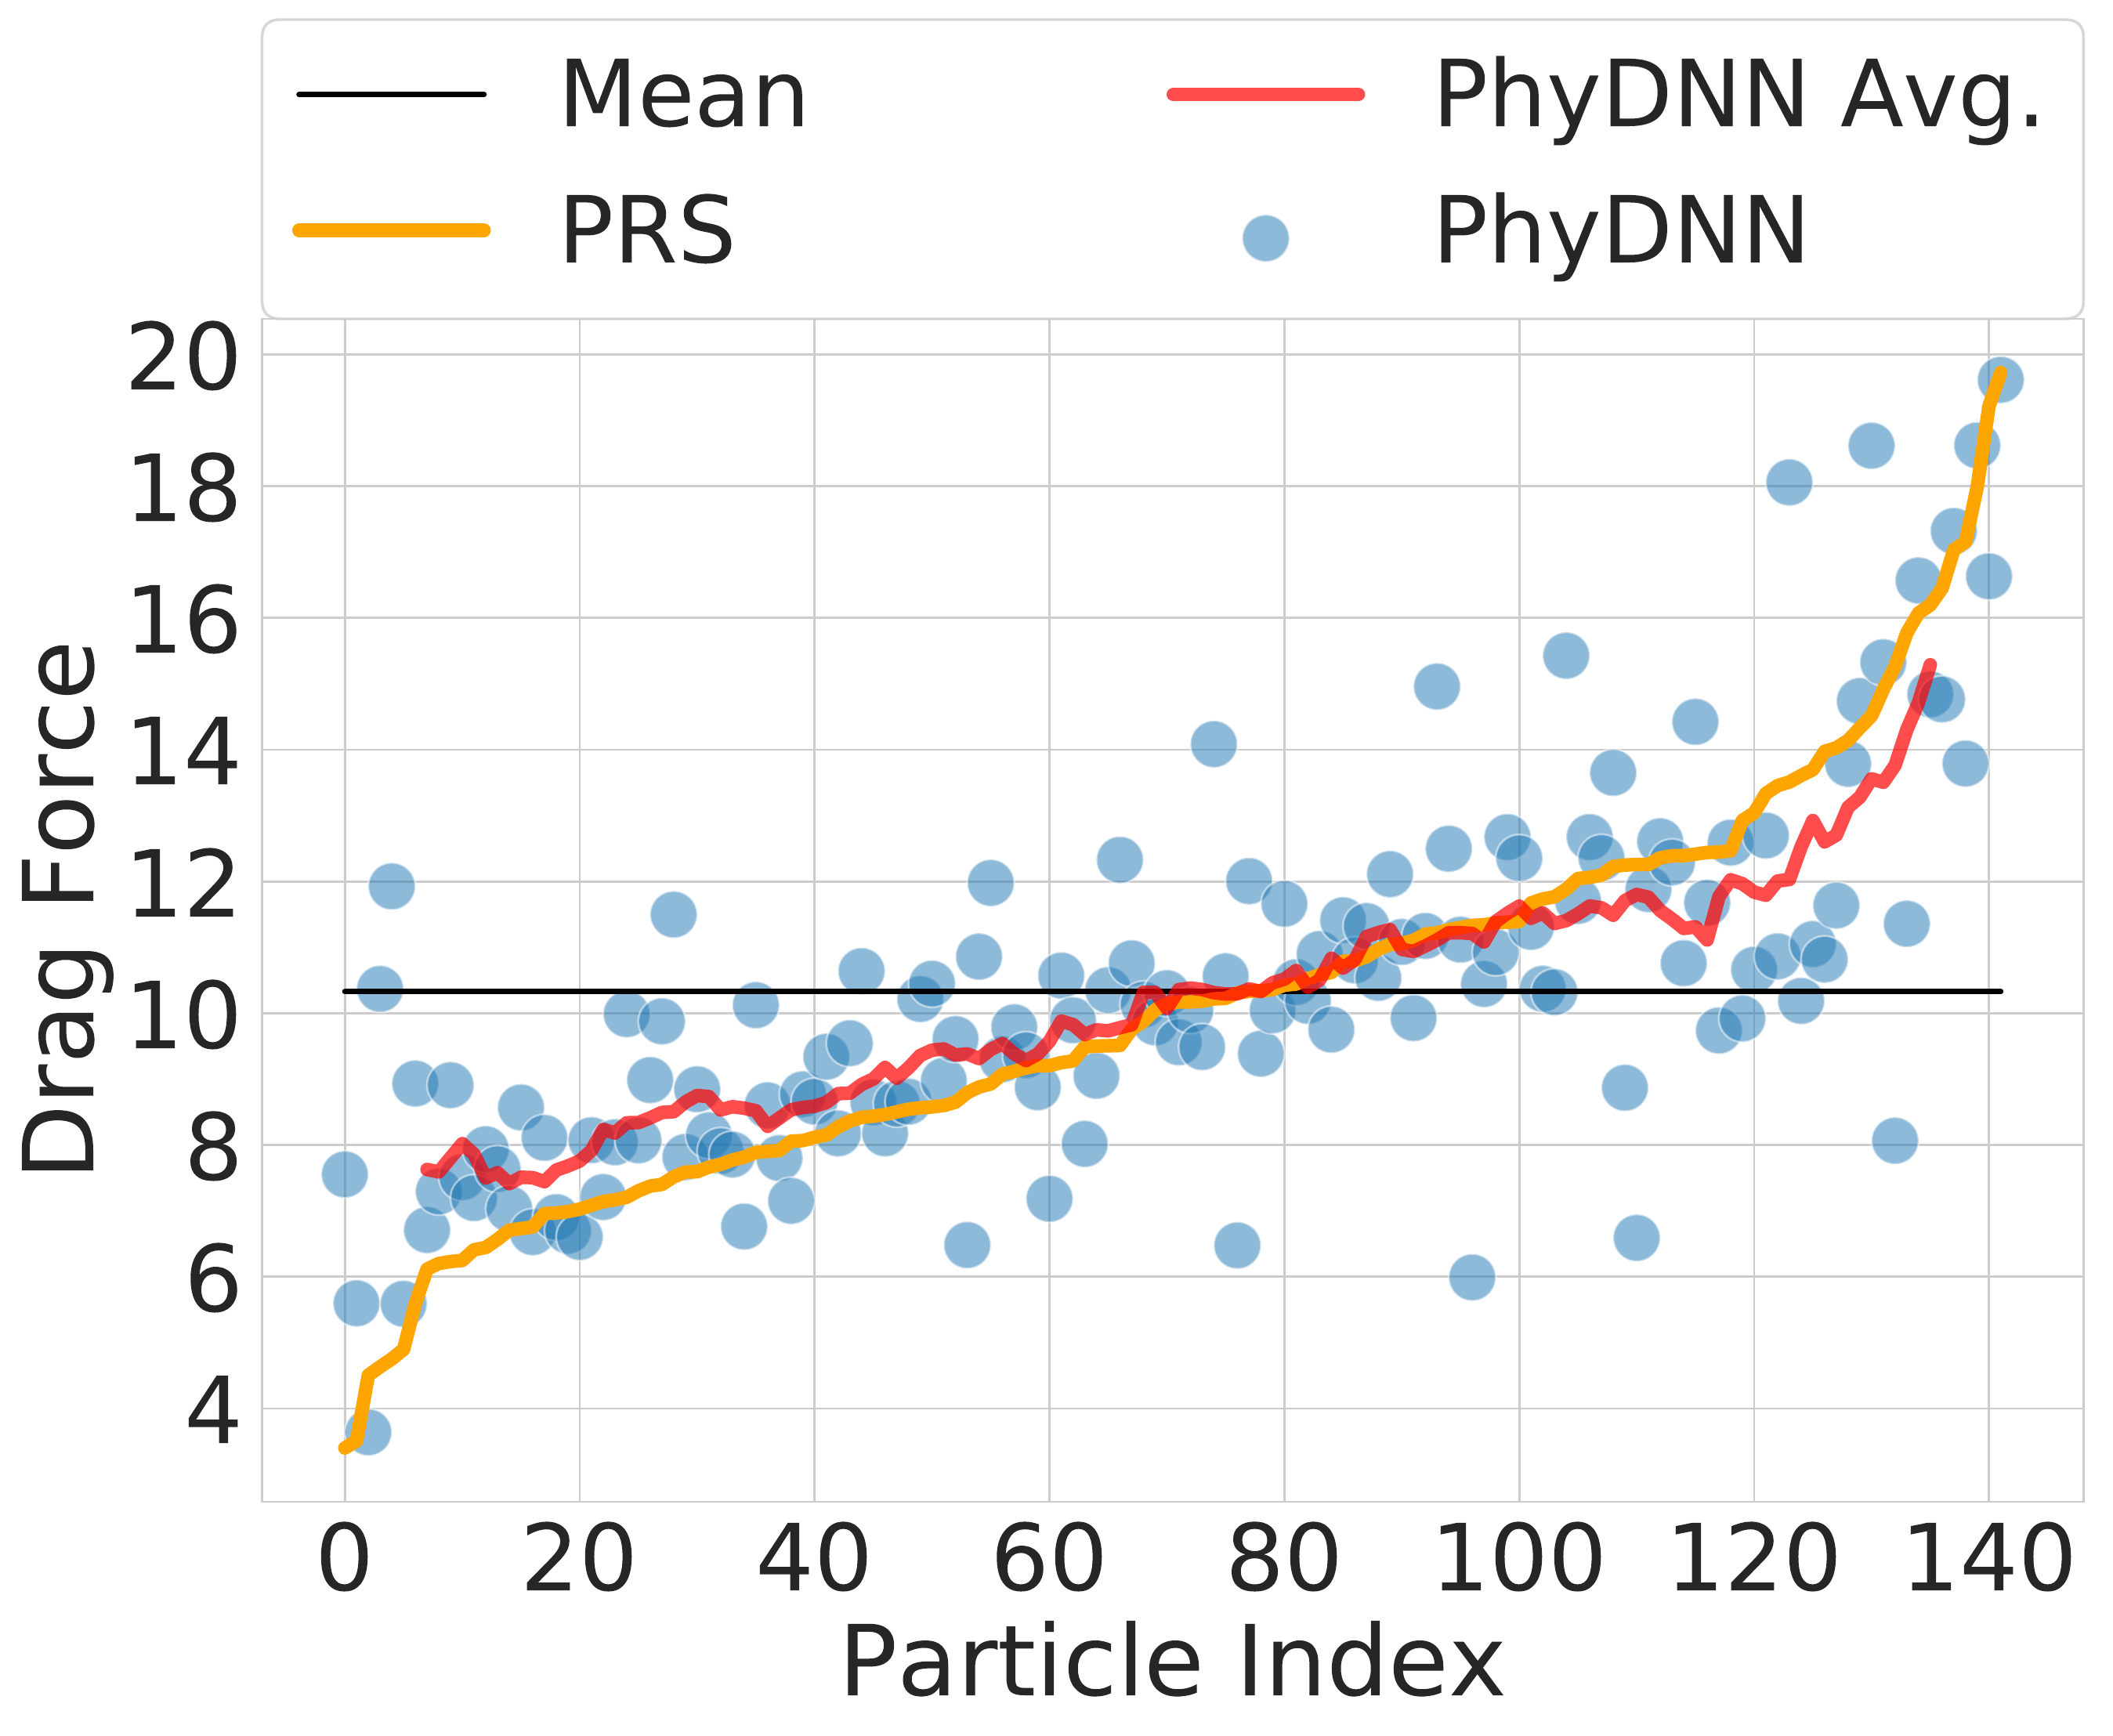}
         \caption{$Re = 50, \phi = 0.2$}
         \label{fig:re_50_sf_20}
     \end{subfigure}
     \hfill
     \begin{subfigure}[b]{0.48\columnwidth}             
         \includegraphics[width=\textwidth]{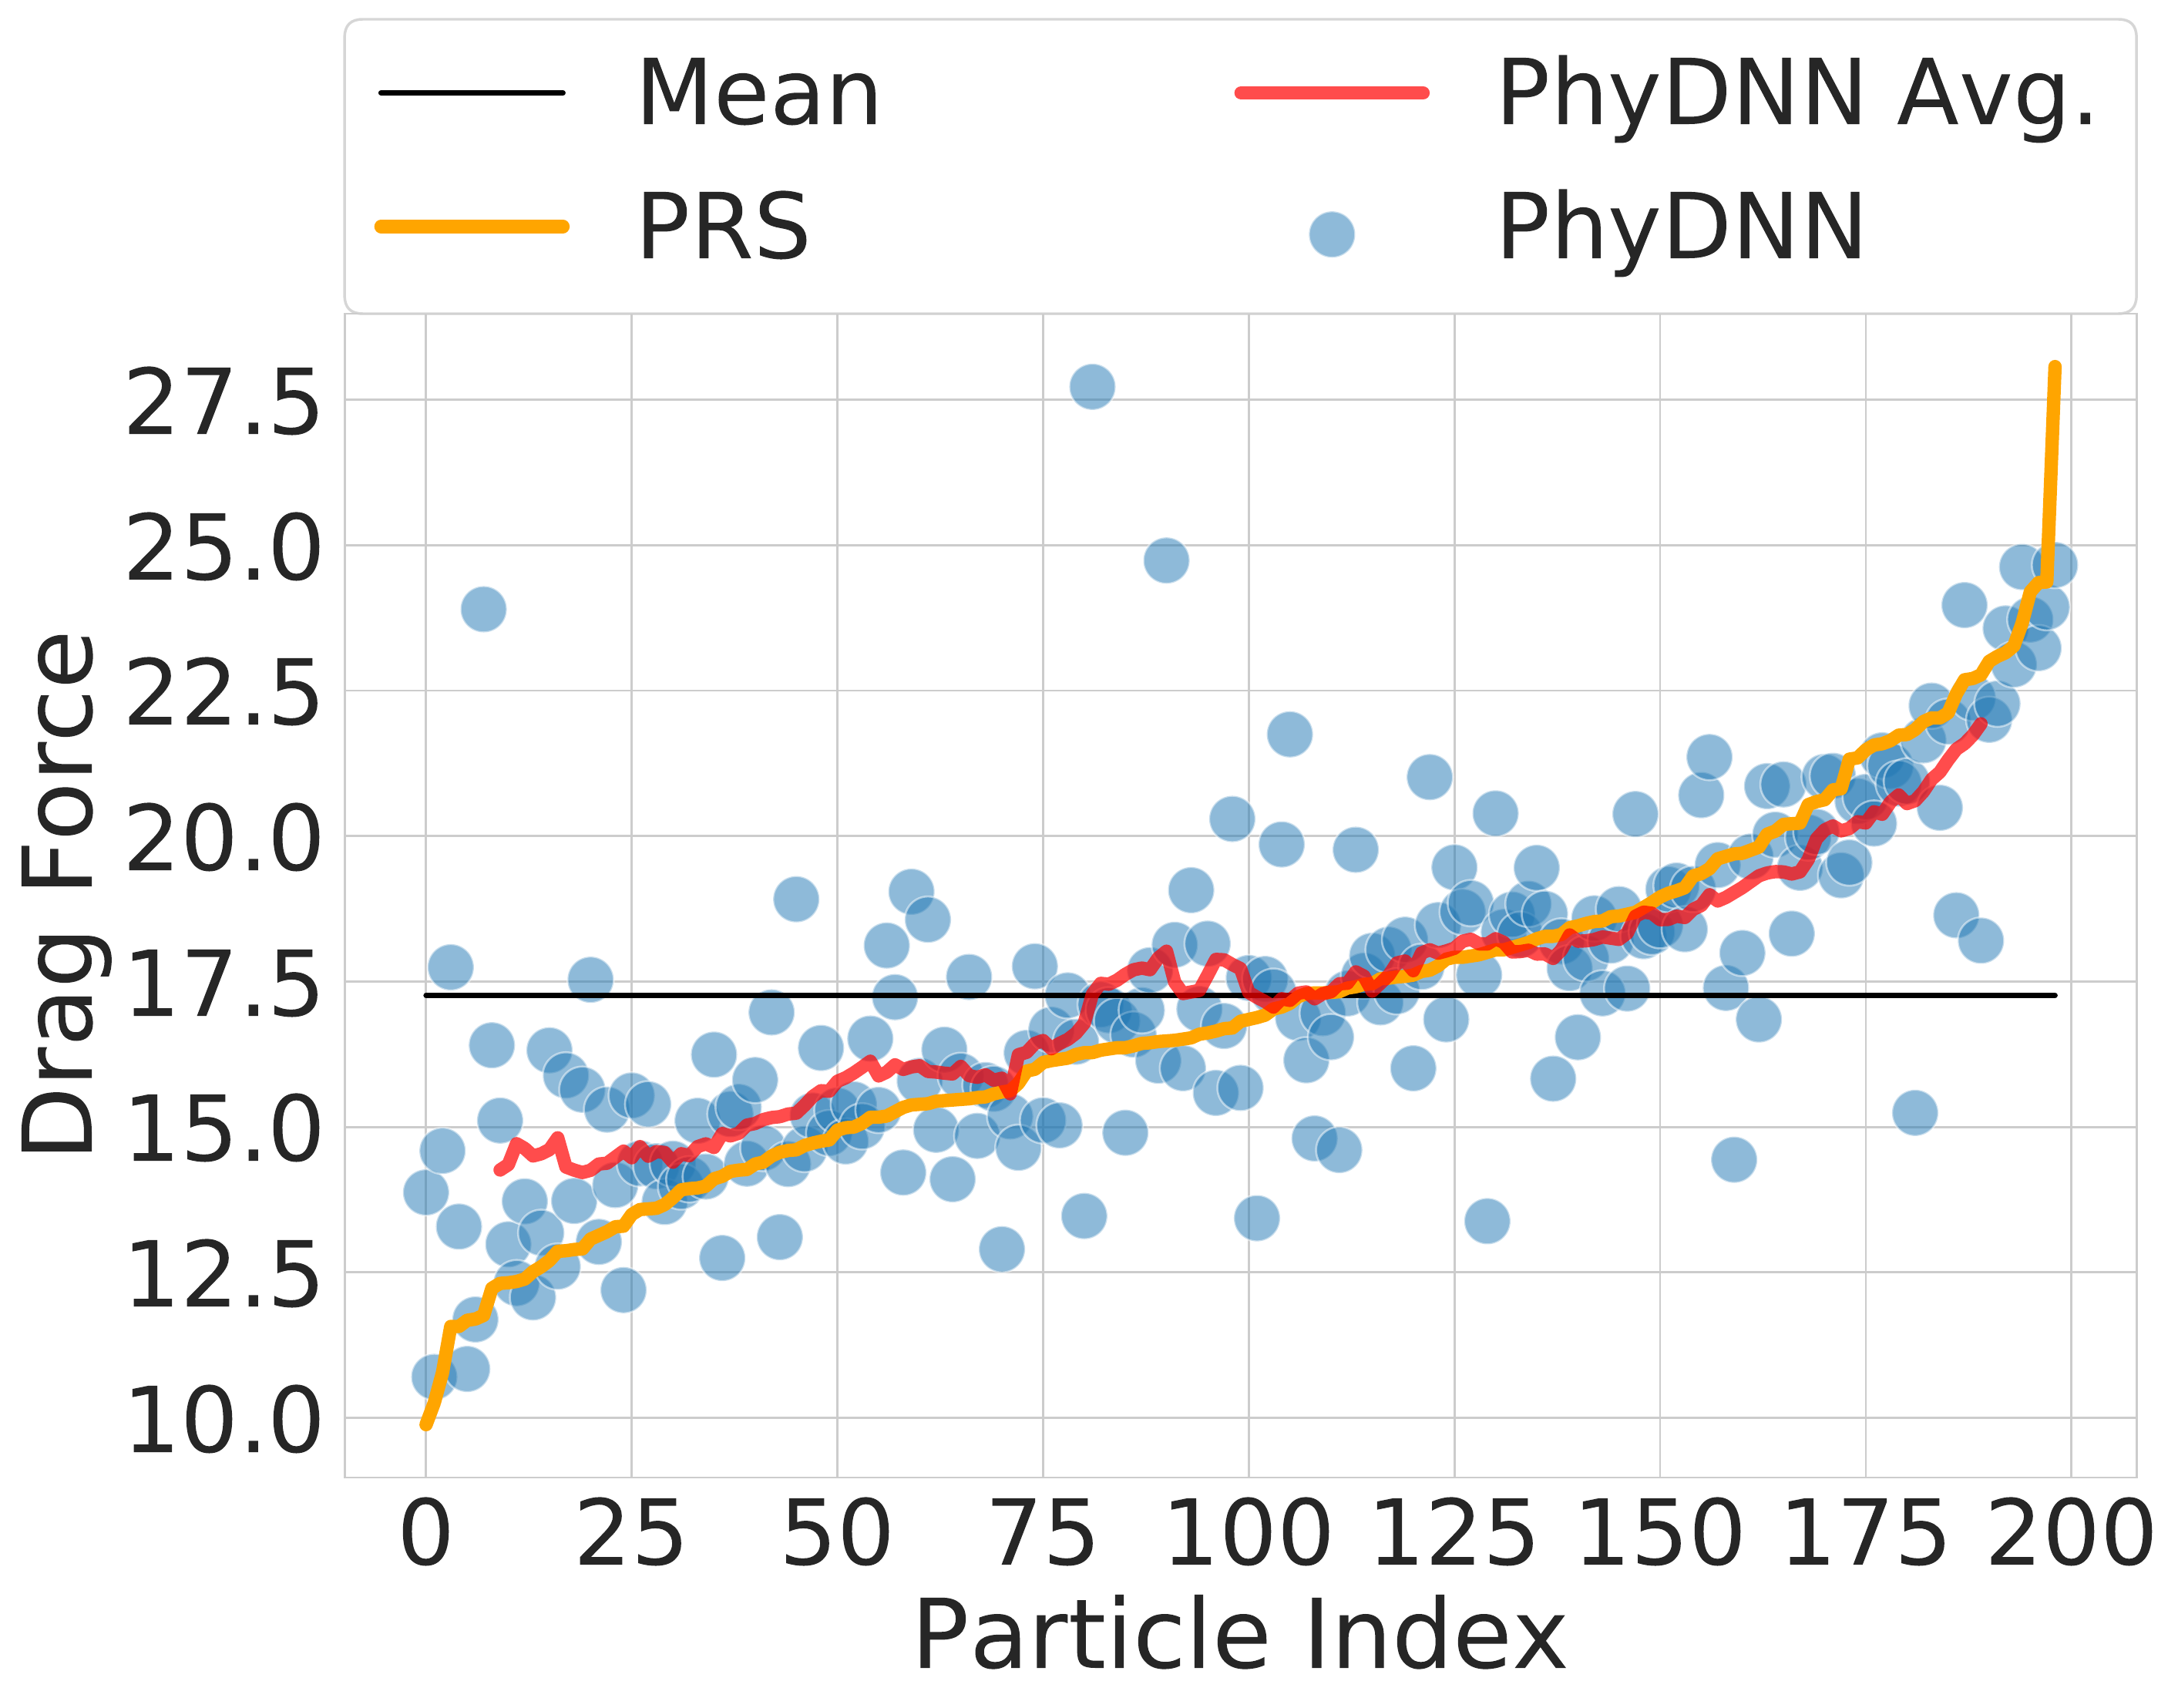}
         \caption{$Re = 50, \phi = 0.3$}
         \label{fig:re_50_sf_30}
     \end{subfigure}
     \hfill
     \begin{subfigure}[b]{0.48\columnwidth}
         \centering
         \includegraphics[width=\textwidth]{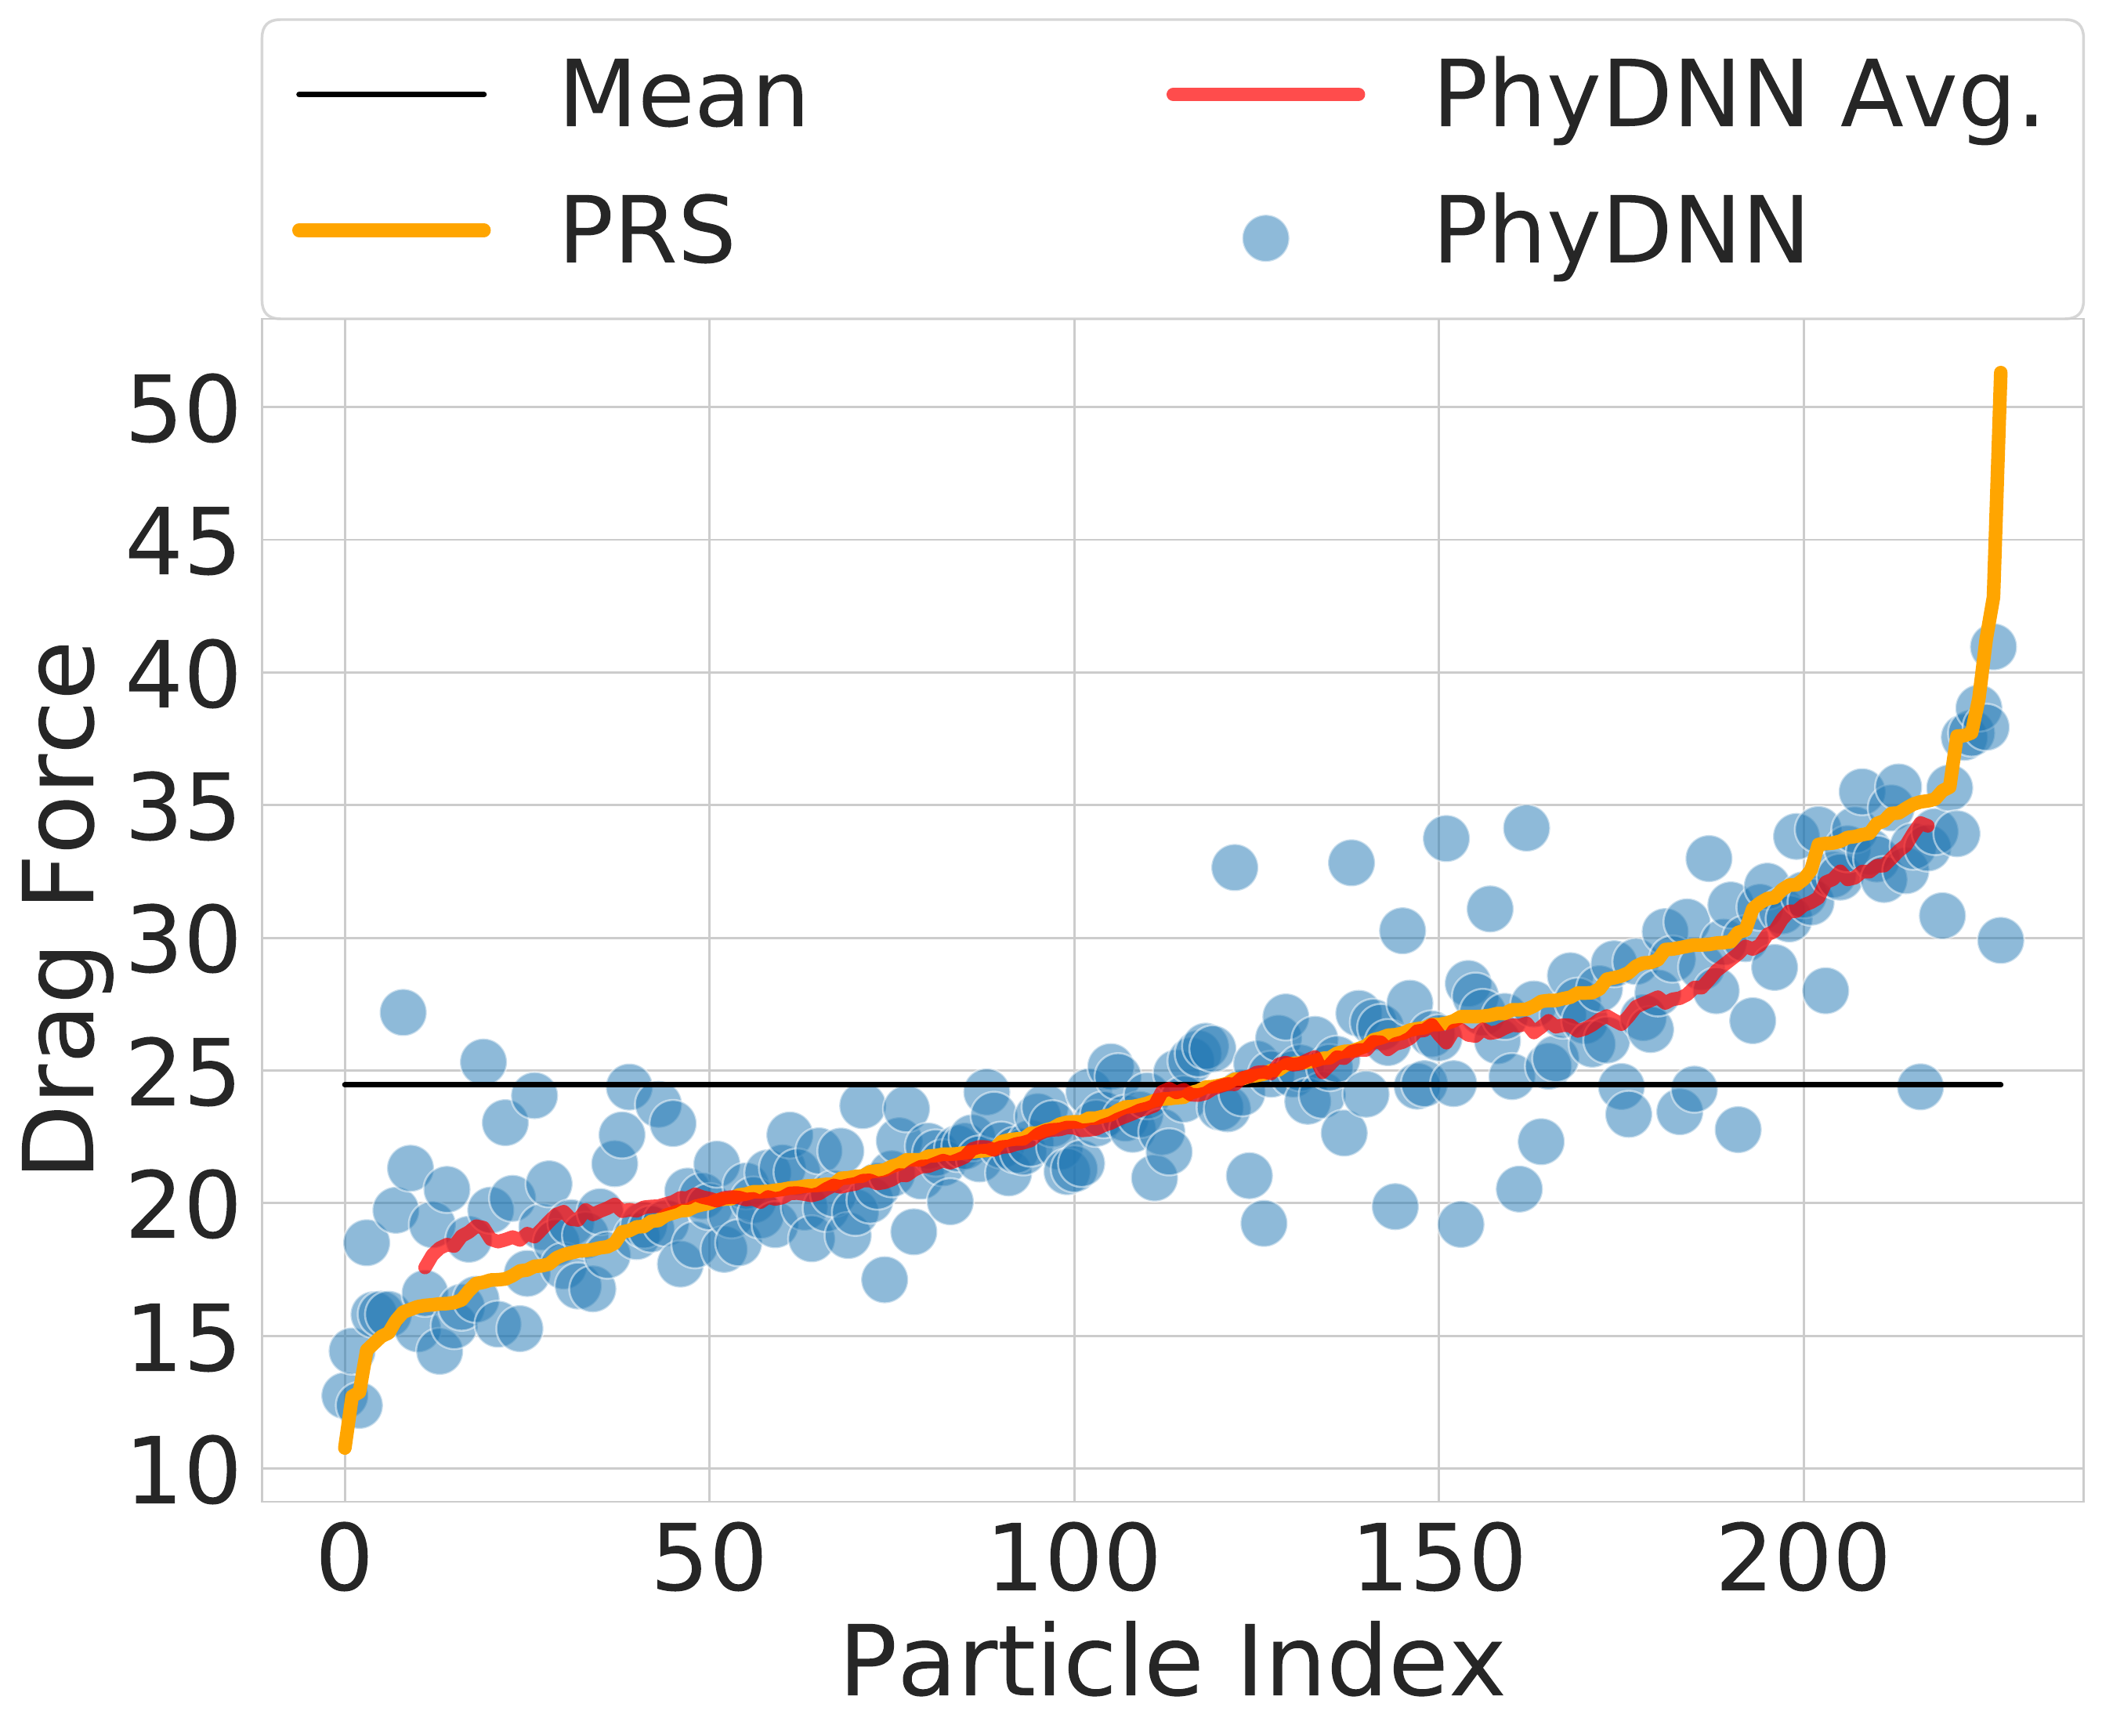}
         \caption{$Re = 50, \phi = 0.35$}
         \label{fig:re_50_sf_35}
     \end{subfigure}
     \vfill %%%%%%%%%%%%%%%%%%%%%%%%%%%%%%%%%%%%%%%%%%%%%%%%%%%%%%%%%%%%%%%%%%%%%%%%%%%%%%%%%%%%%%%%%%%%
    \begin{subfigure}[b]{0.48\columnwidth}         
         \includegraphics[width=\textwidth]{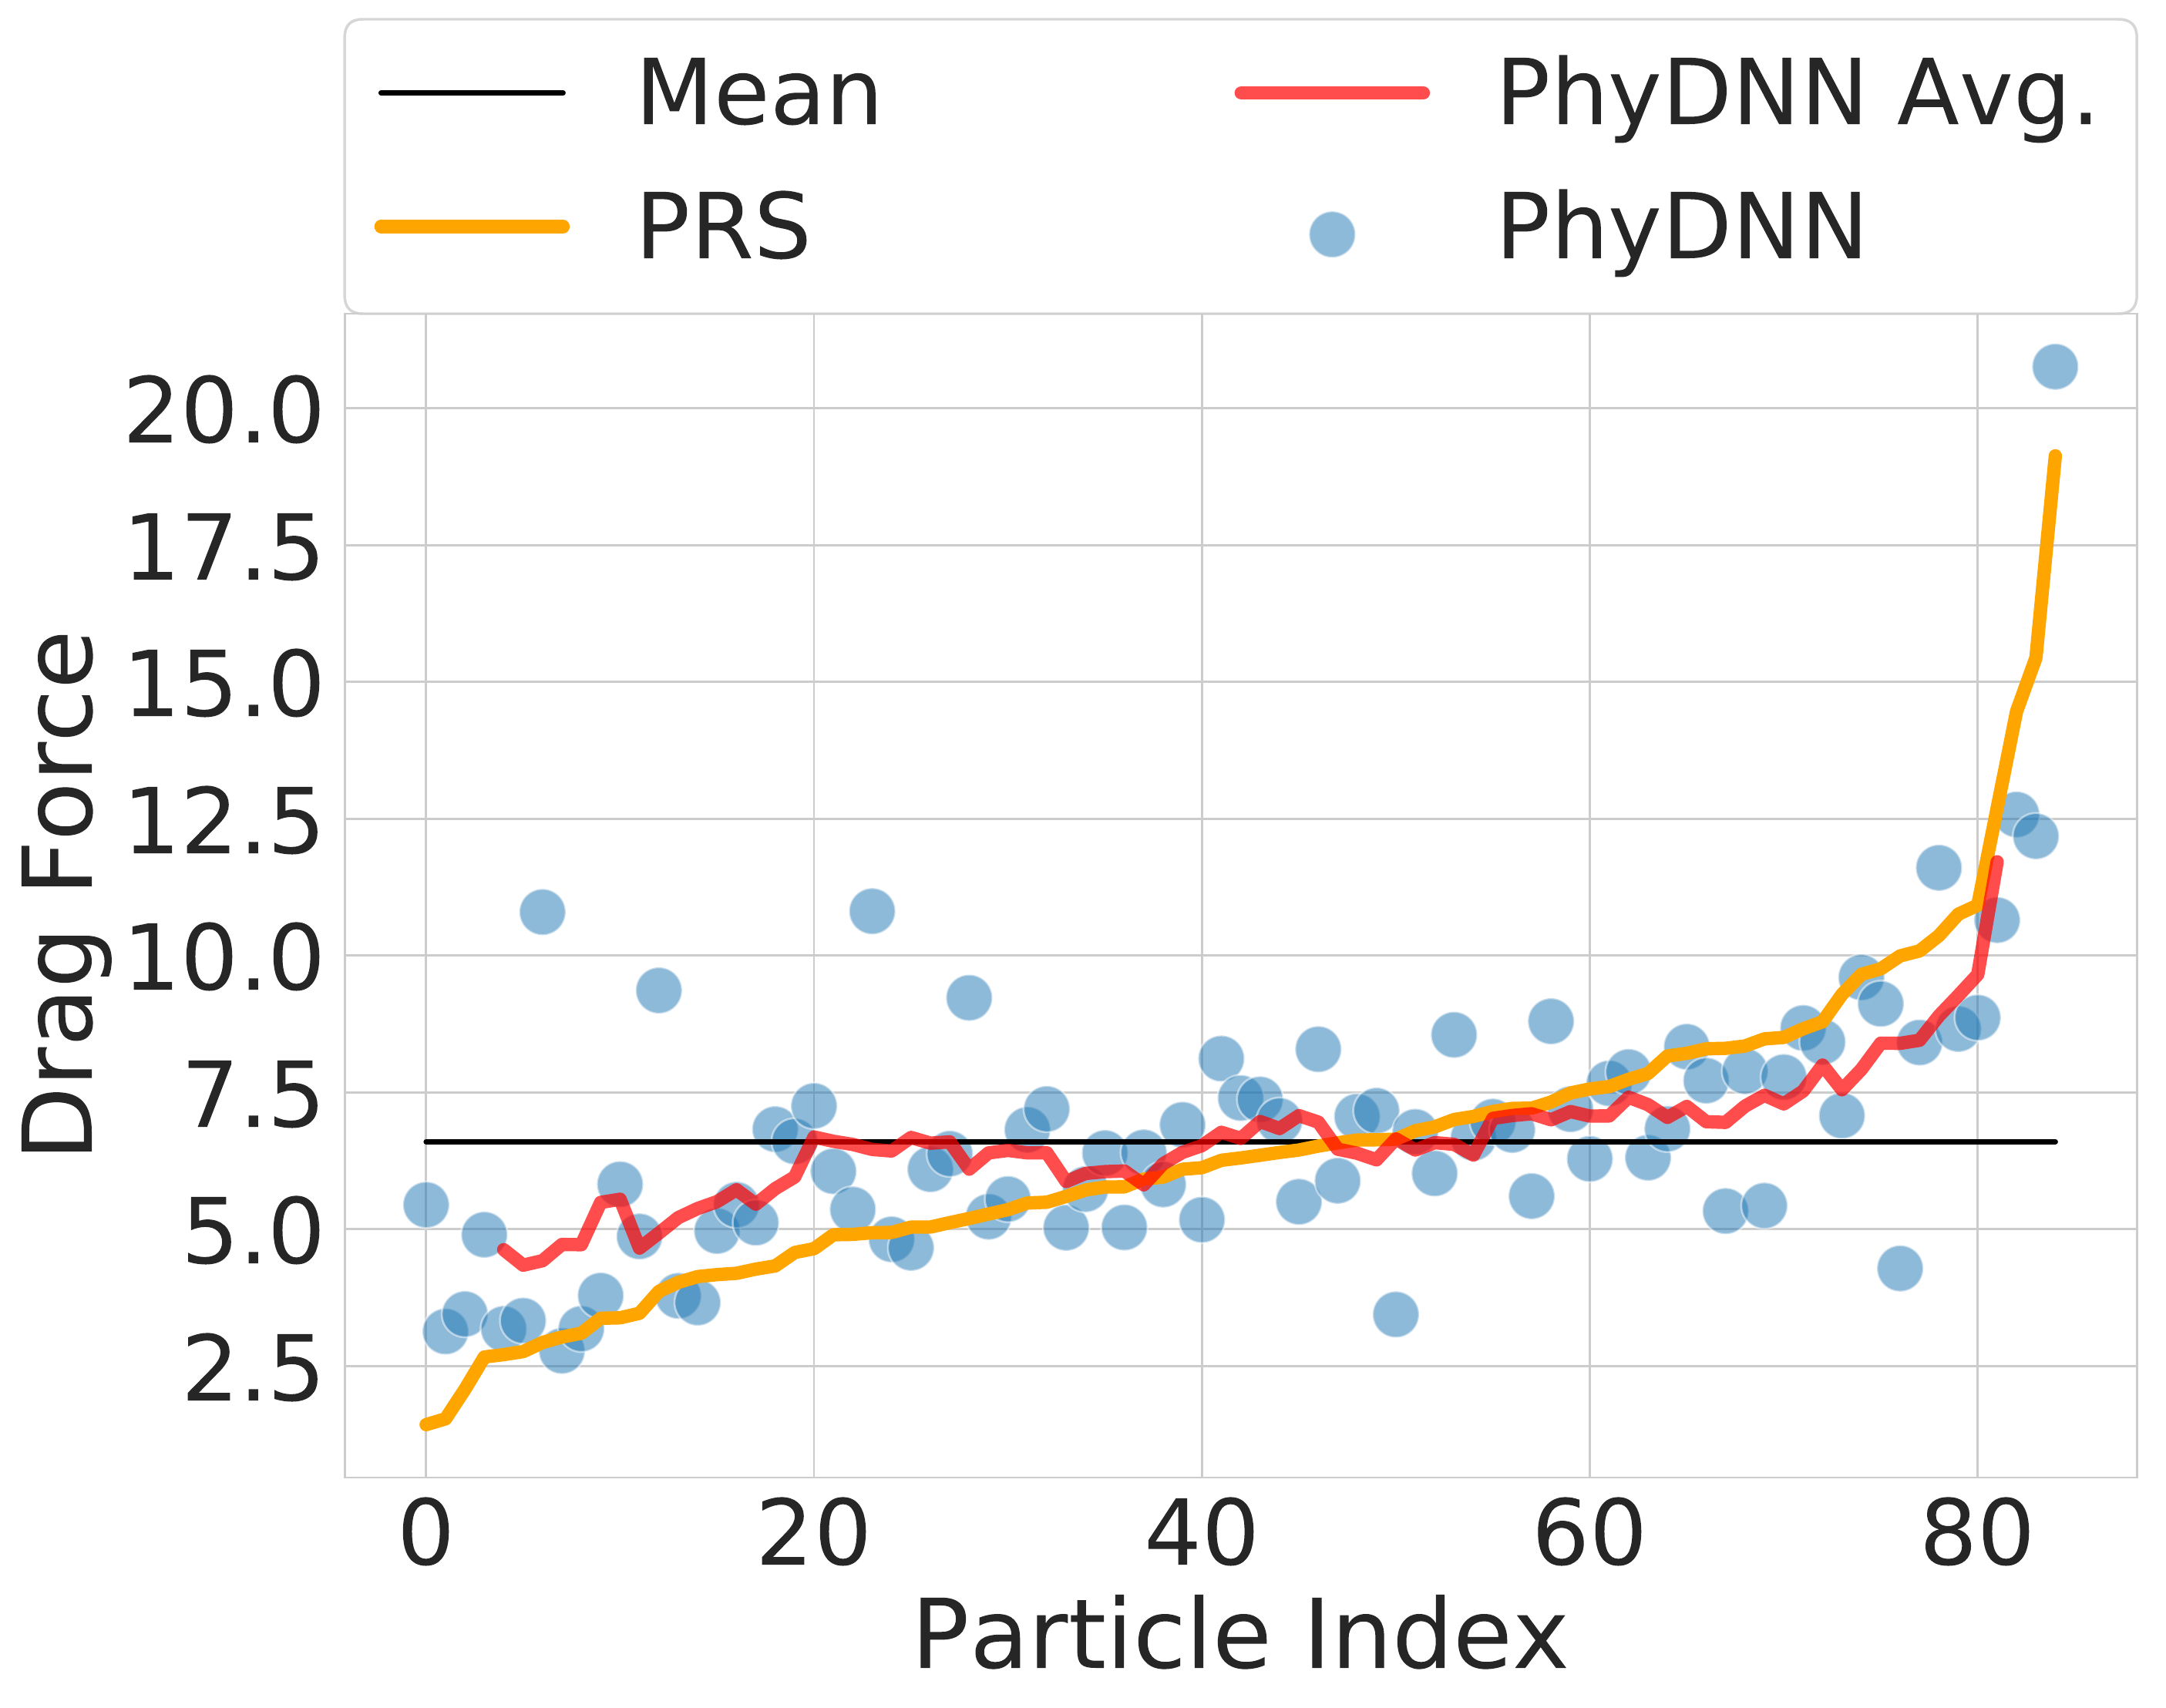}
         \caption{$Re = 100, \phi = 0.1$}
         \label{fig:re_100_sf_10}
     \end{subfigure}
     \hfill
     \begin{subfigure}[b]{0.48\columnwidth}
         \centering
         \includegraphics[width=\textwidth]{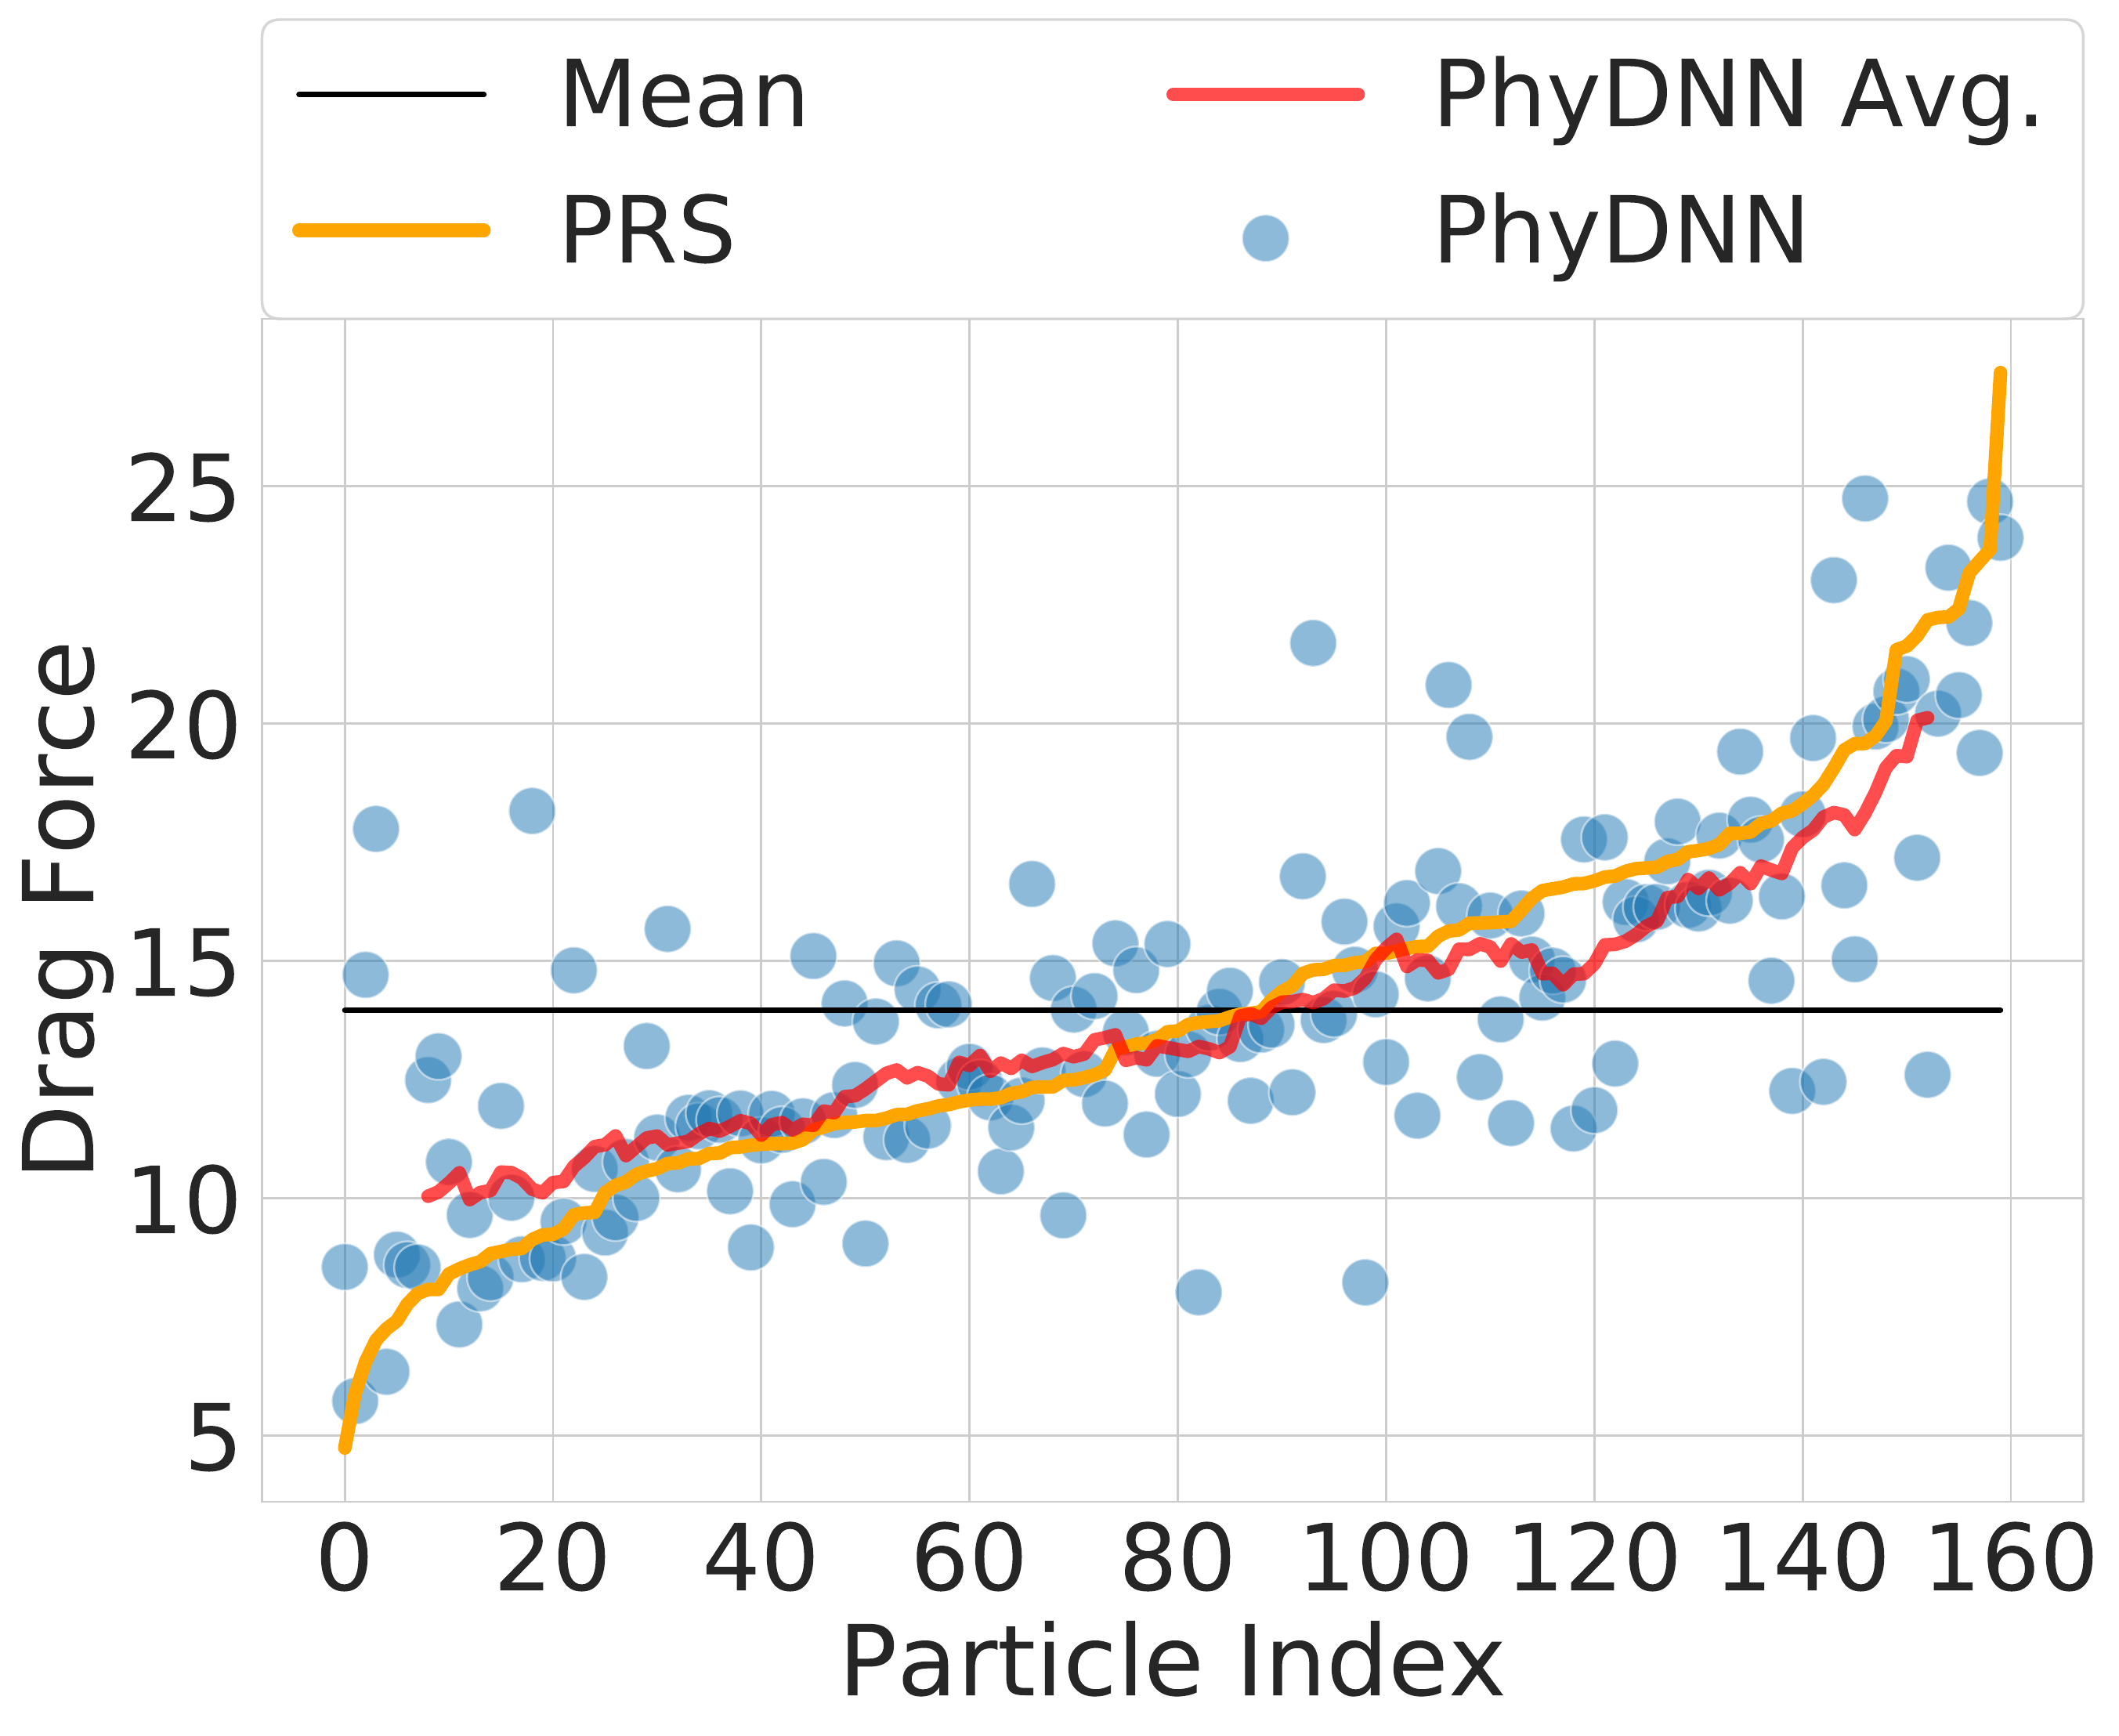}
         \caption{$Re = 100, \phi = 0.2$}
         \label{fig:re_100_sf_20}
     \end{subfigure}
     \hfill
     \begin{subfigure}[b]{0.48\columnwidth}             
         \includegraphics[width=\textwidth]{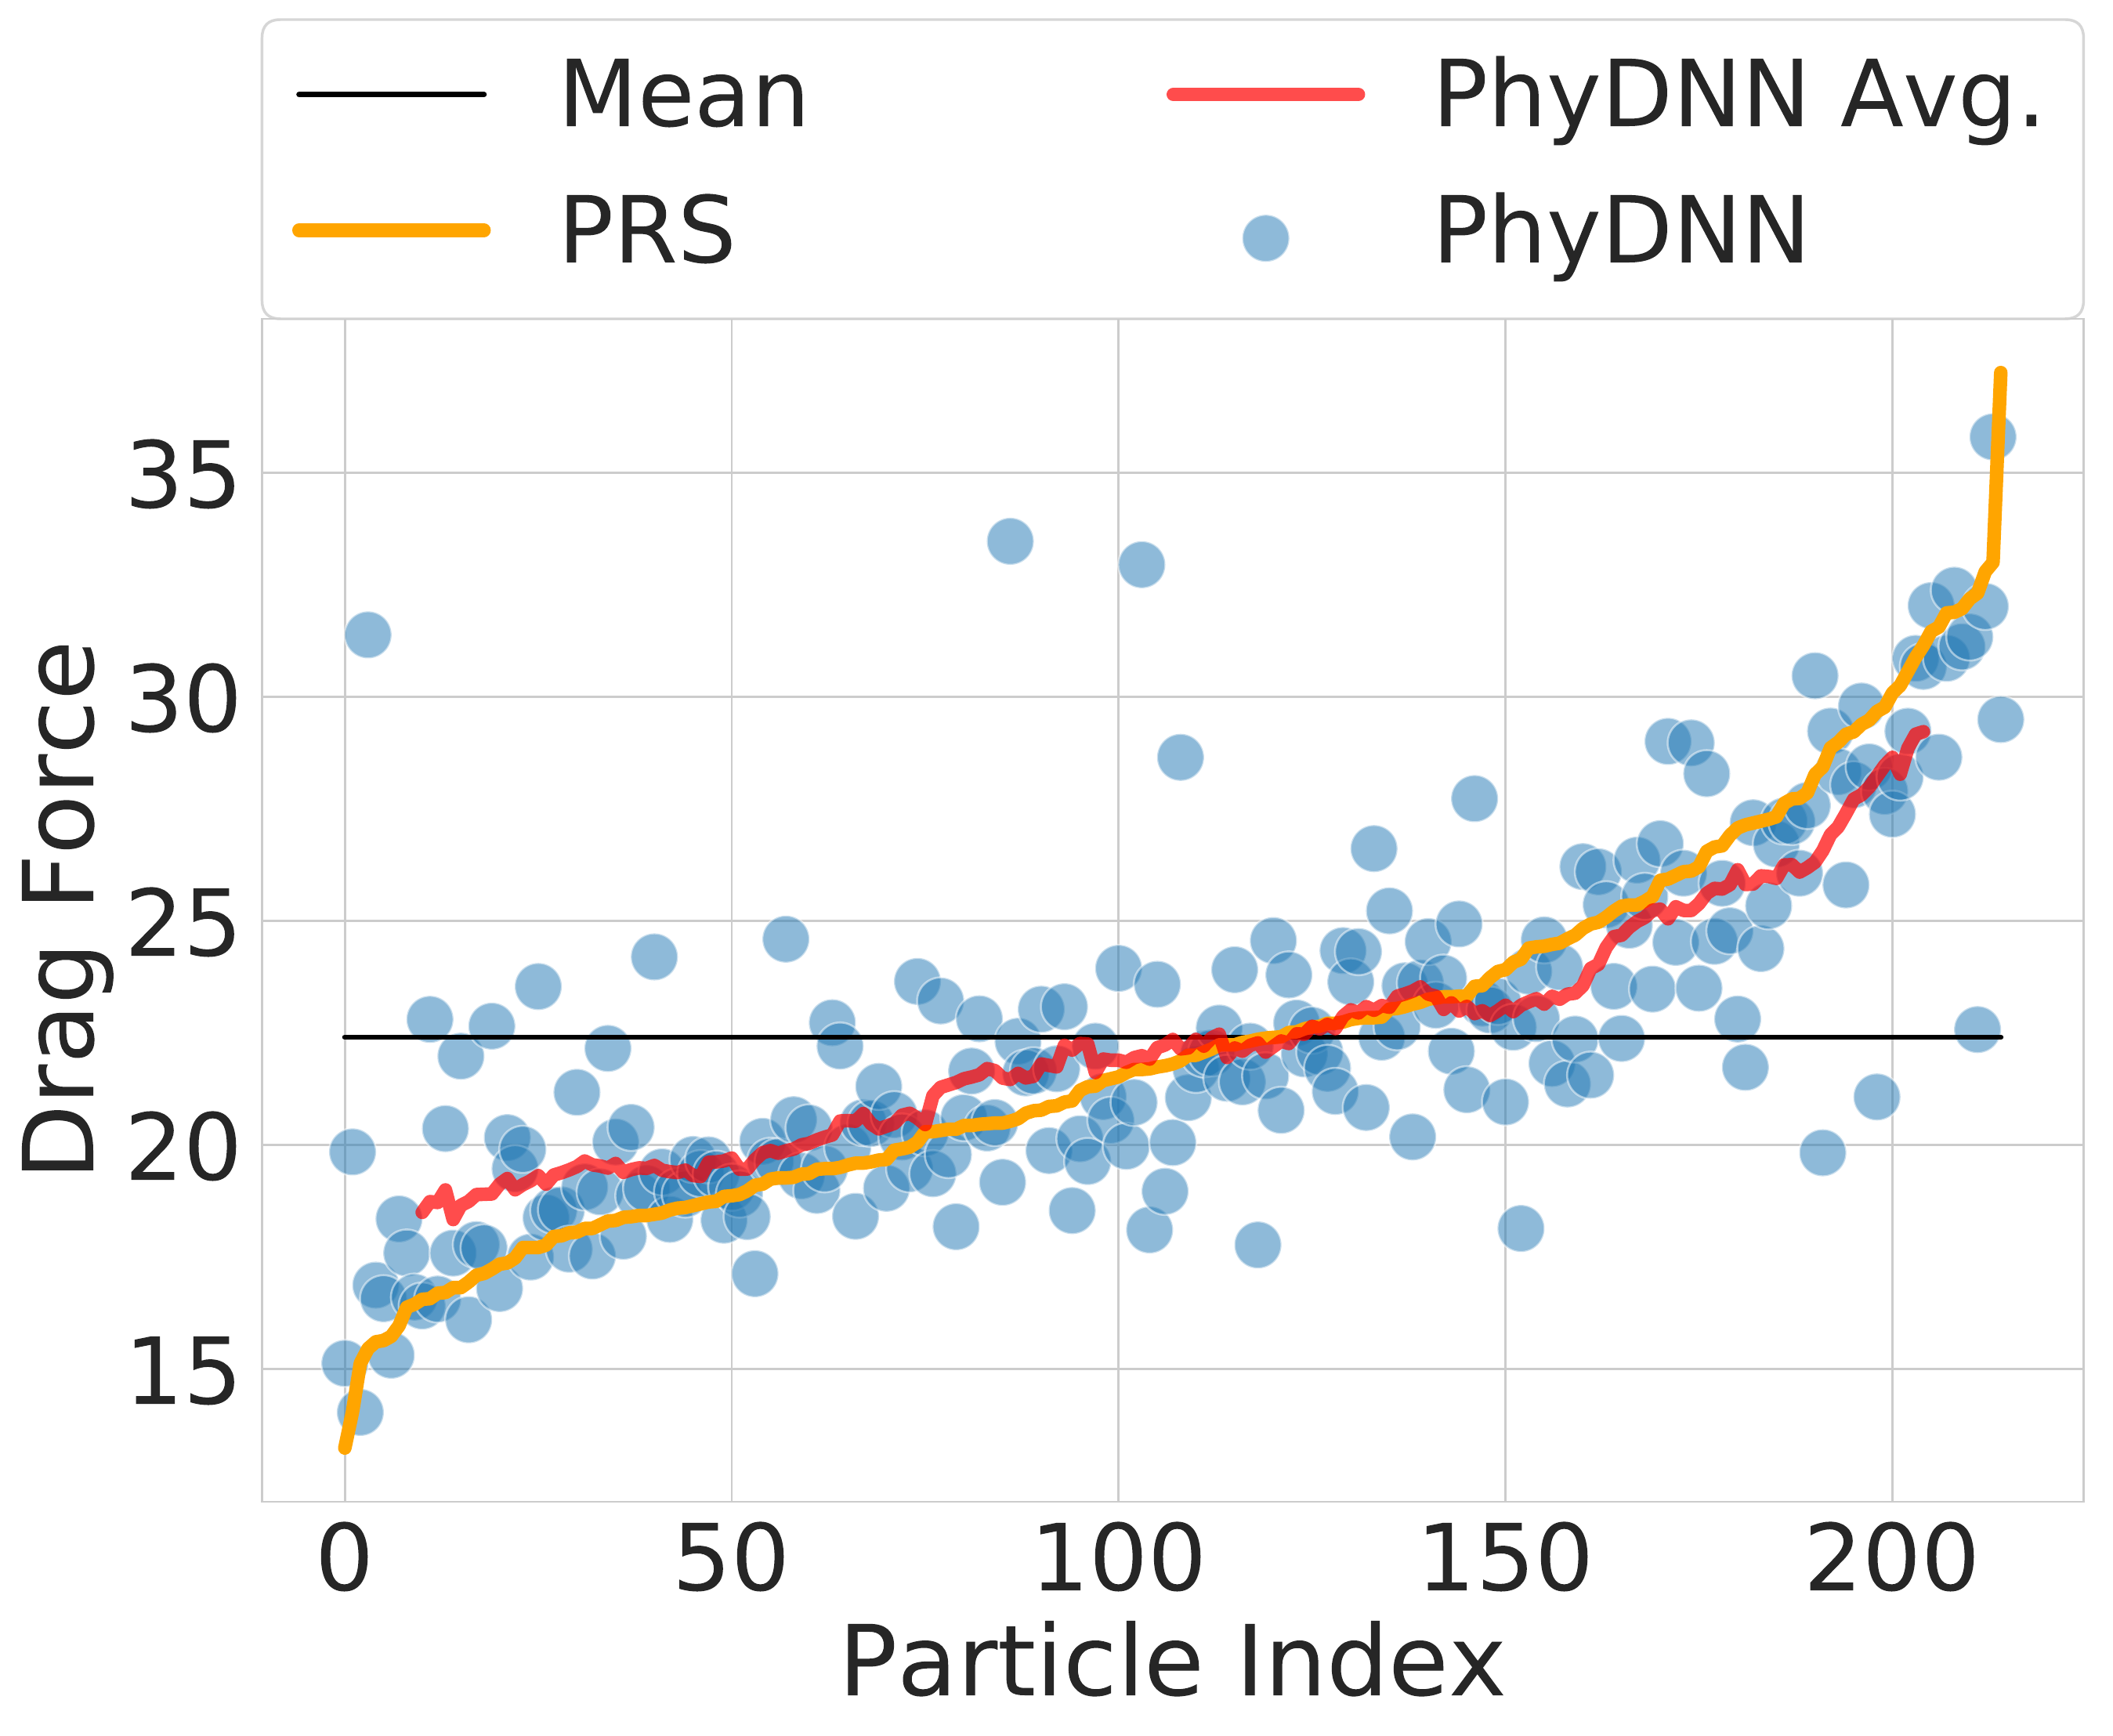}
         \caption{$Re = 100, \phi = 0.3$}
         \label{fig:re_100_sf_30}
     \end{subfigure}
     \hfill
     \begin{subfigure}[b]{0.48\columnwidth}
         \centering
         \includegraphics[width=\textwidth]{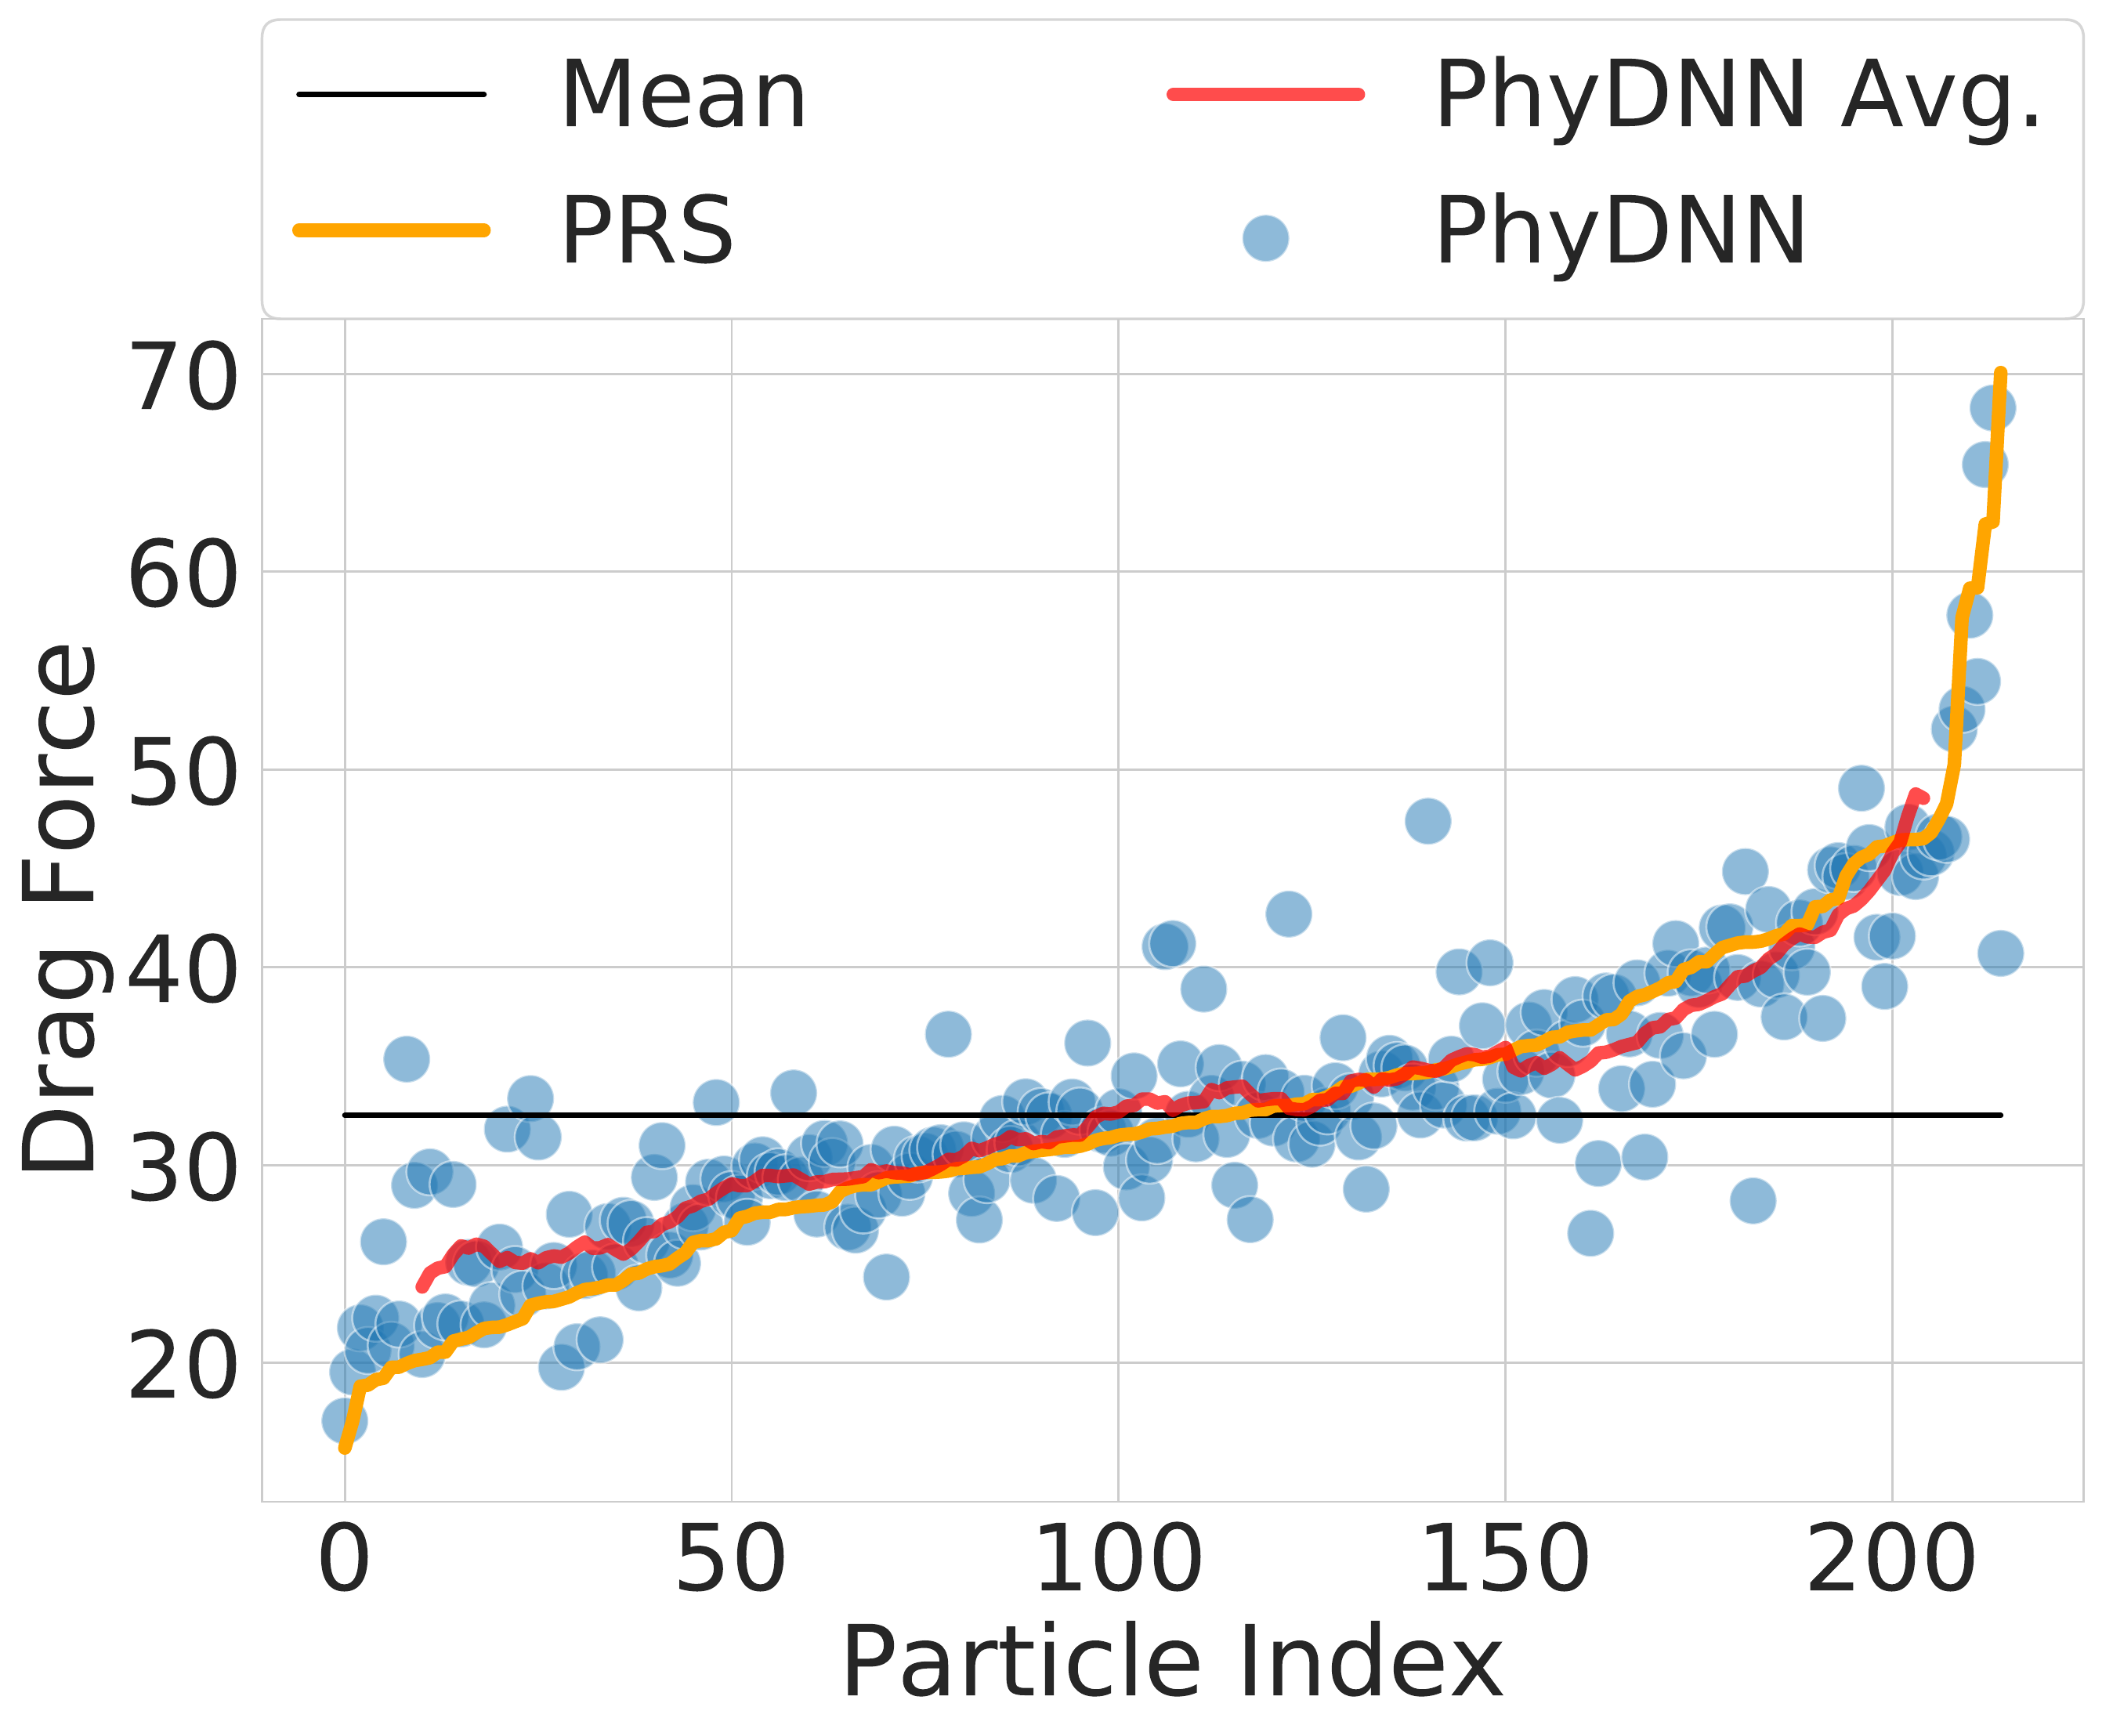}
         \caption{$Re = 100, \phi = 0.35$}
         \label{fig:re_100_sf_35}
     \end{subfigure}
     \vfill %%%%%%%%%%%%%%%%%%%%%%%%%%%%%%%%%%%%%%%%%%%%%%%%%%%%%%%%%%%%%%%%%%%%%%%%%%%%%%%%%%%%%%%%%%%%% 
      \begin{subfigure}[b]{0.48\columnwidth}
         \centering
         \includegraphics[width=\textwidth]{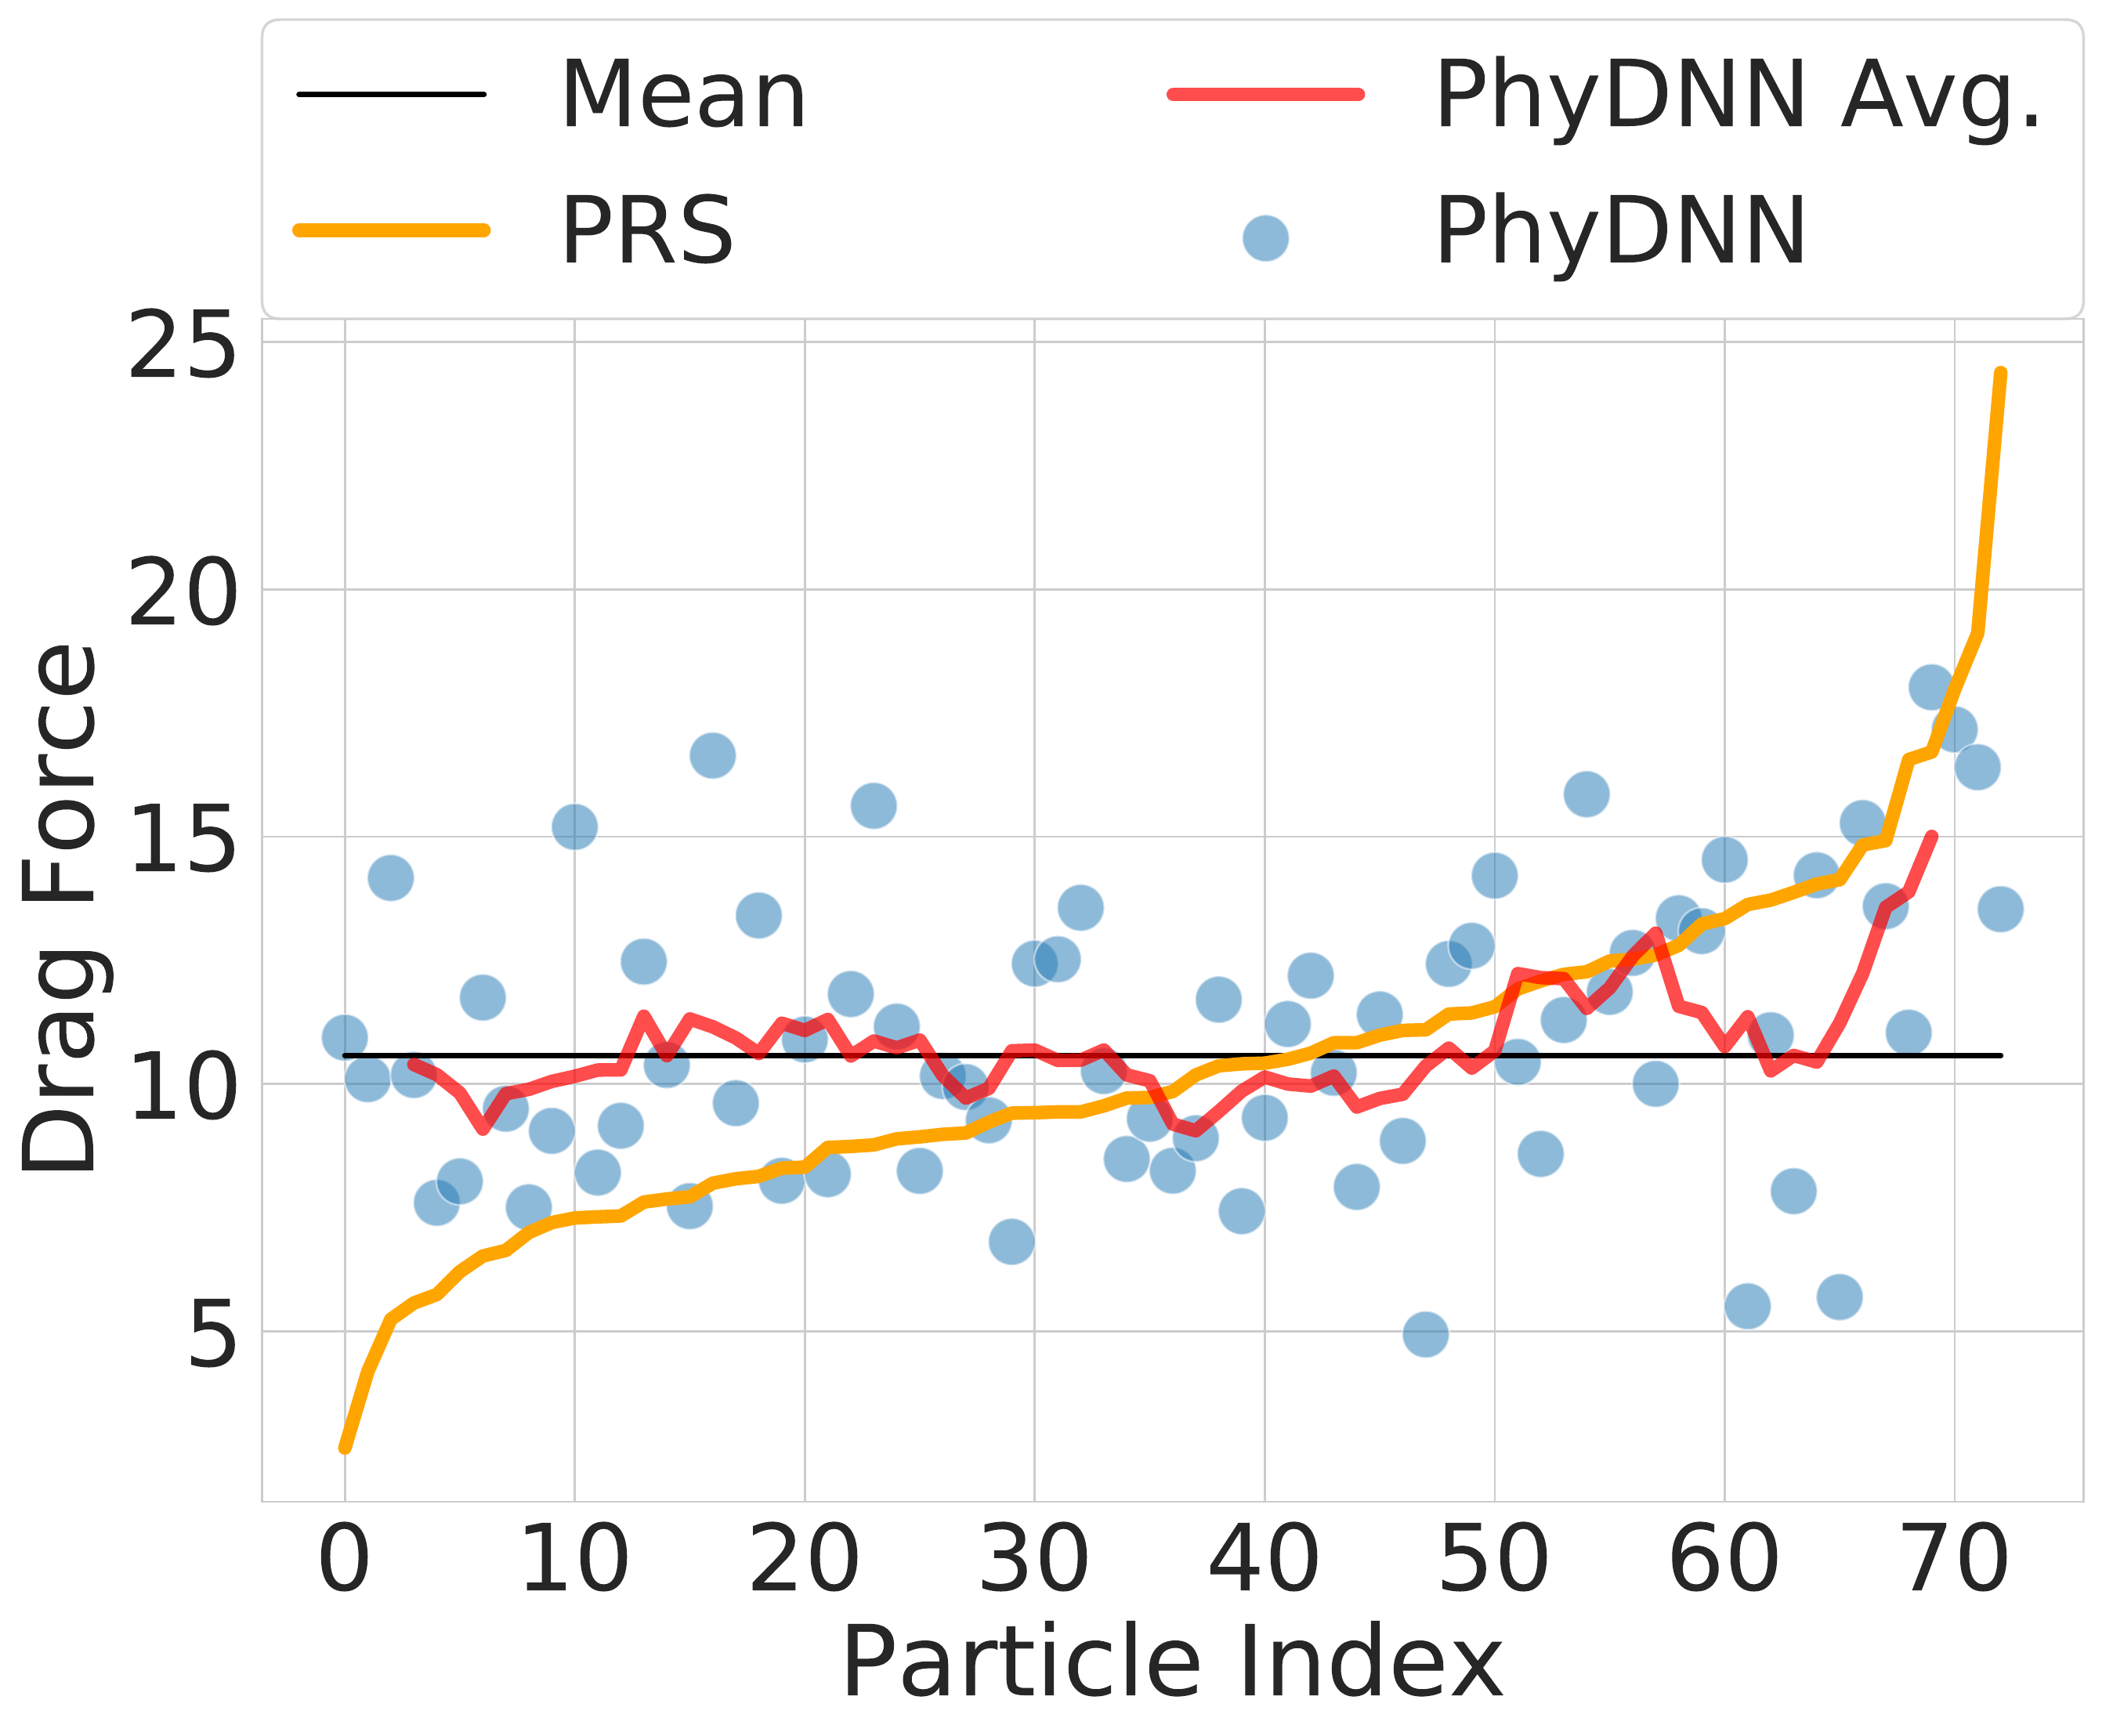}
         \caption{$Re = 200, \phi = 0.1$}
         \label{fig:re_200_sf_10}
     \end{subfigure}
     \hfill
     \begin{subfigure}[b]{0.48\columnwidth}
         \centering
         \includegraphics[width=\textwidth]{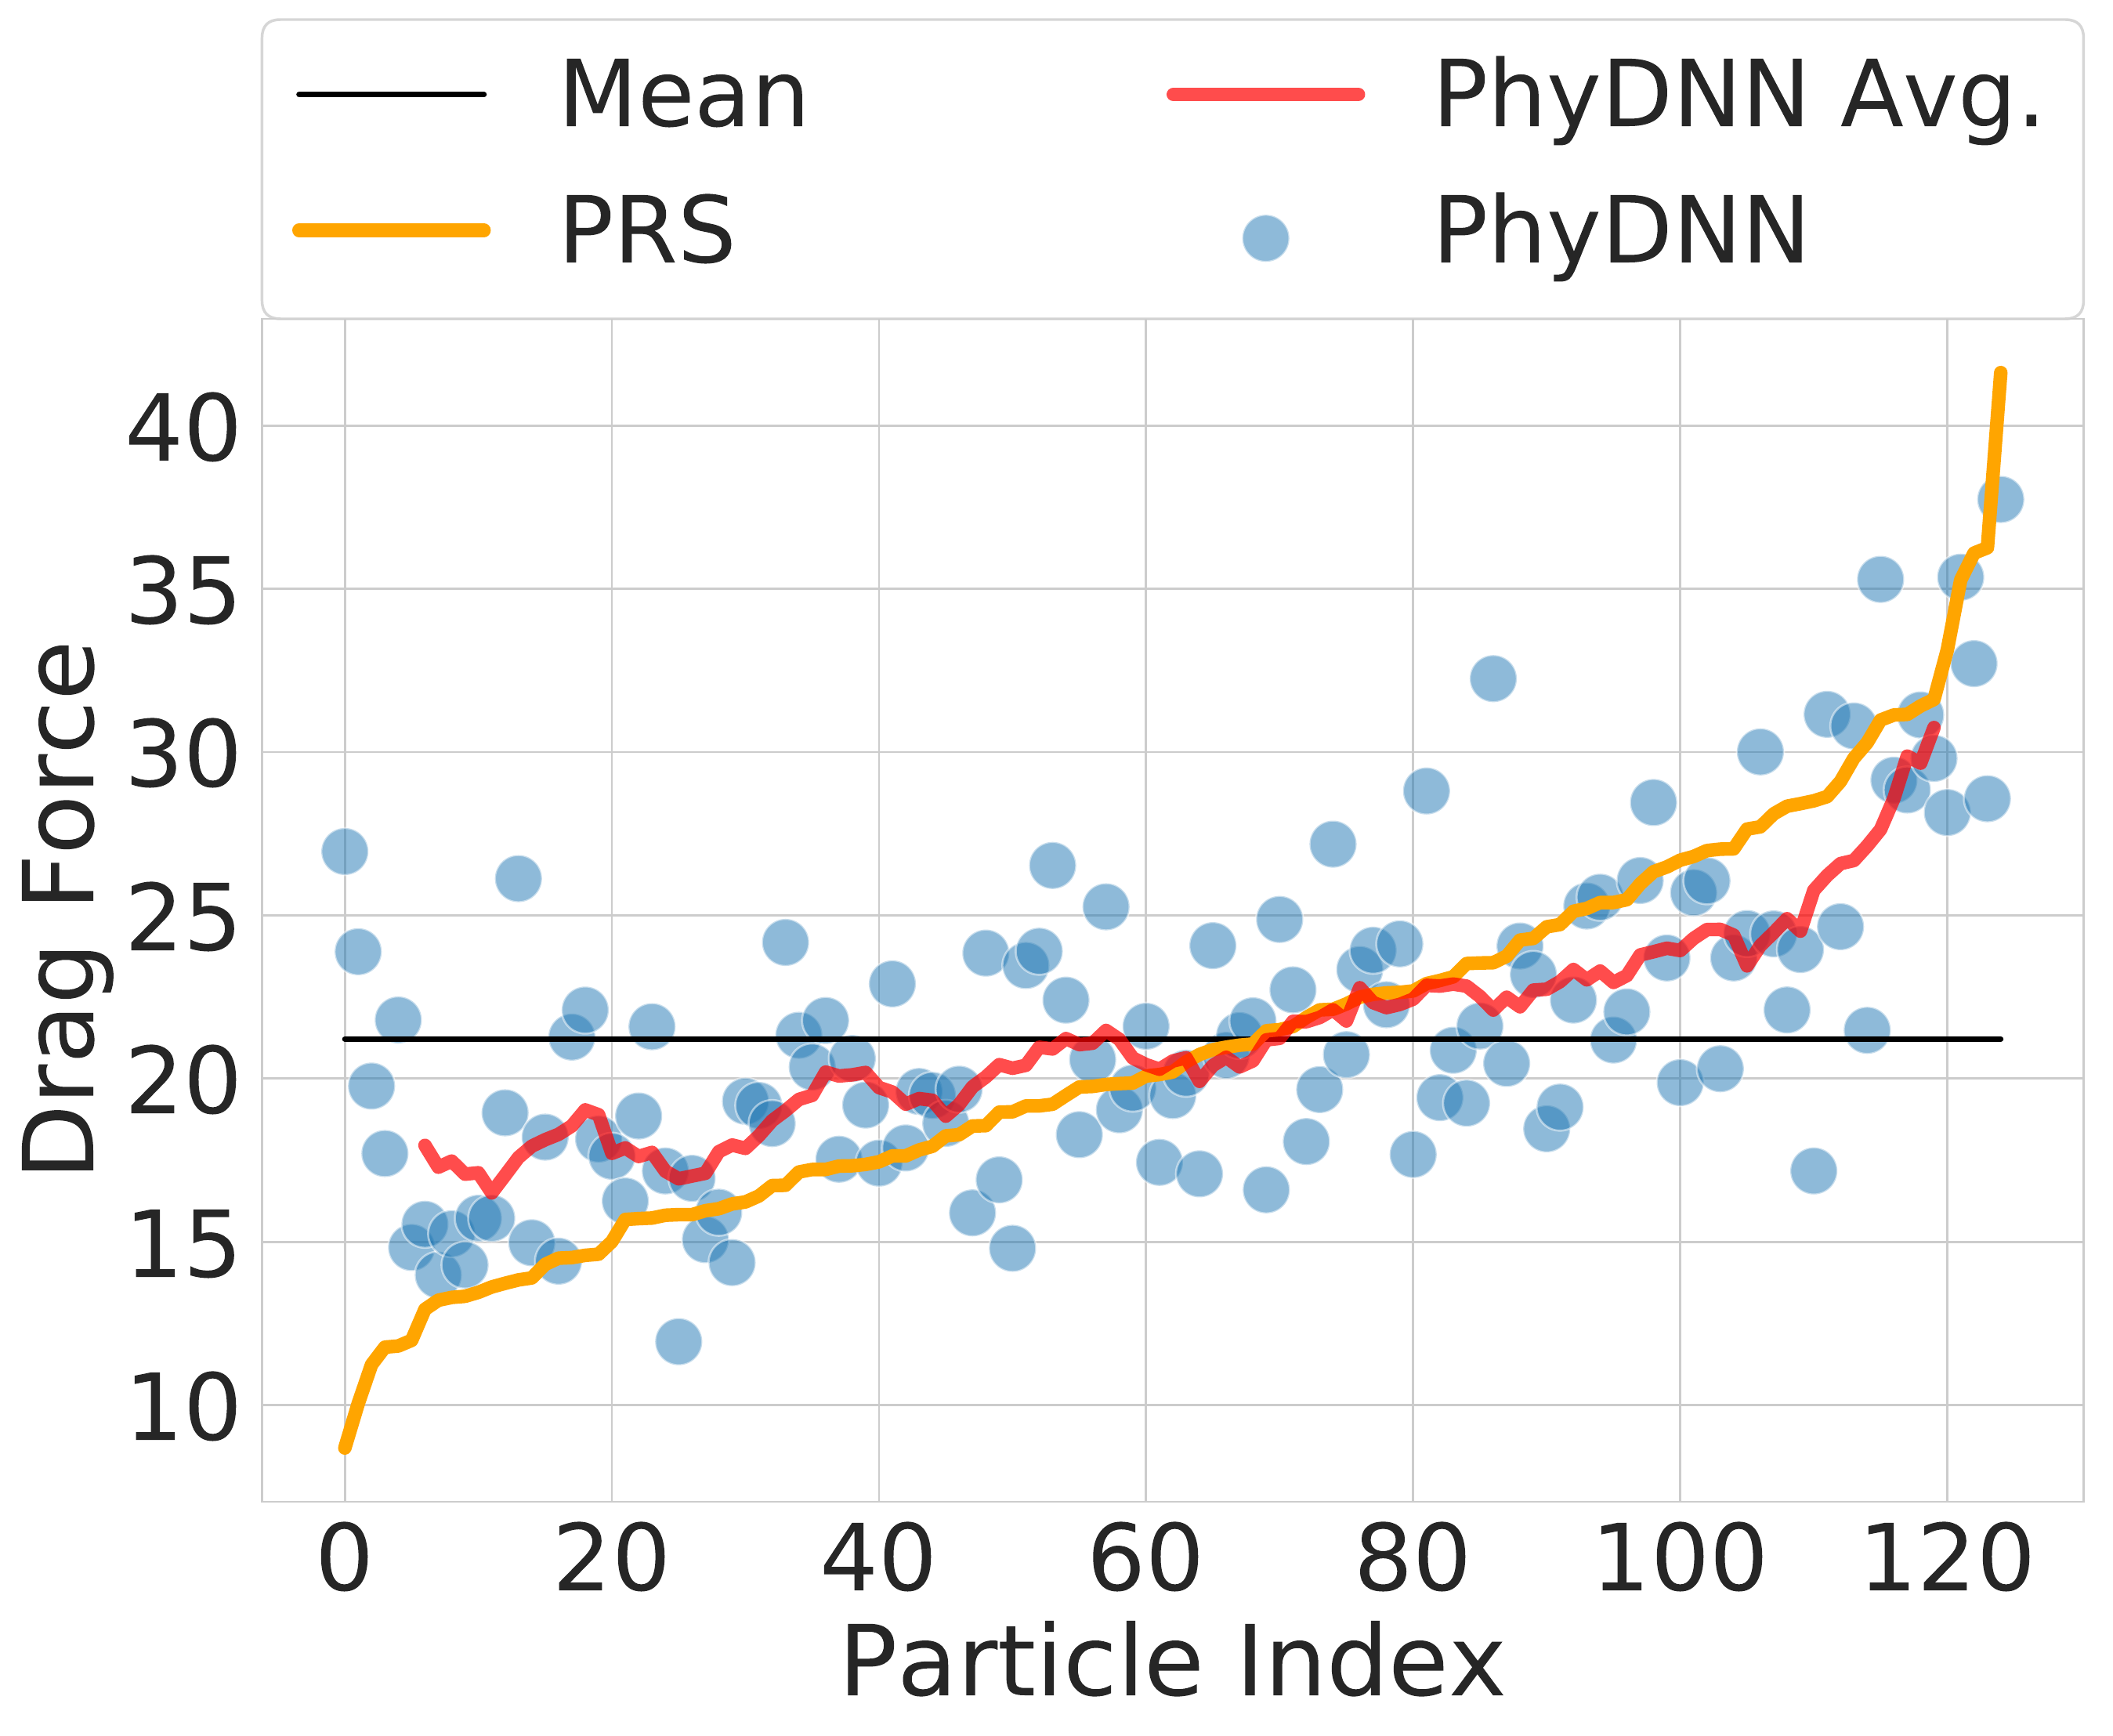}
         \caption{$Re = 200, \phi = 0.2$}
         \label{fig:re_200_sf_20}
     \end{subfigure}
     \hfill
          \begin{subfigure}[b]{0.48\columnwidth}
         \centering
         \includegraphics[width=\textwidth]{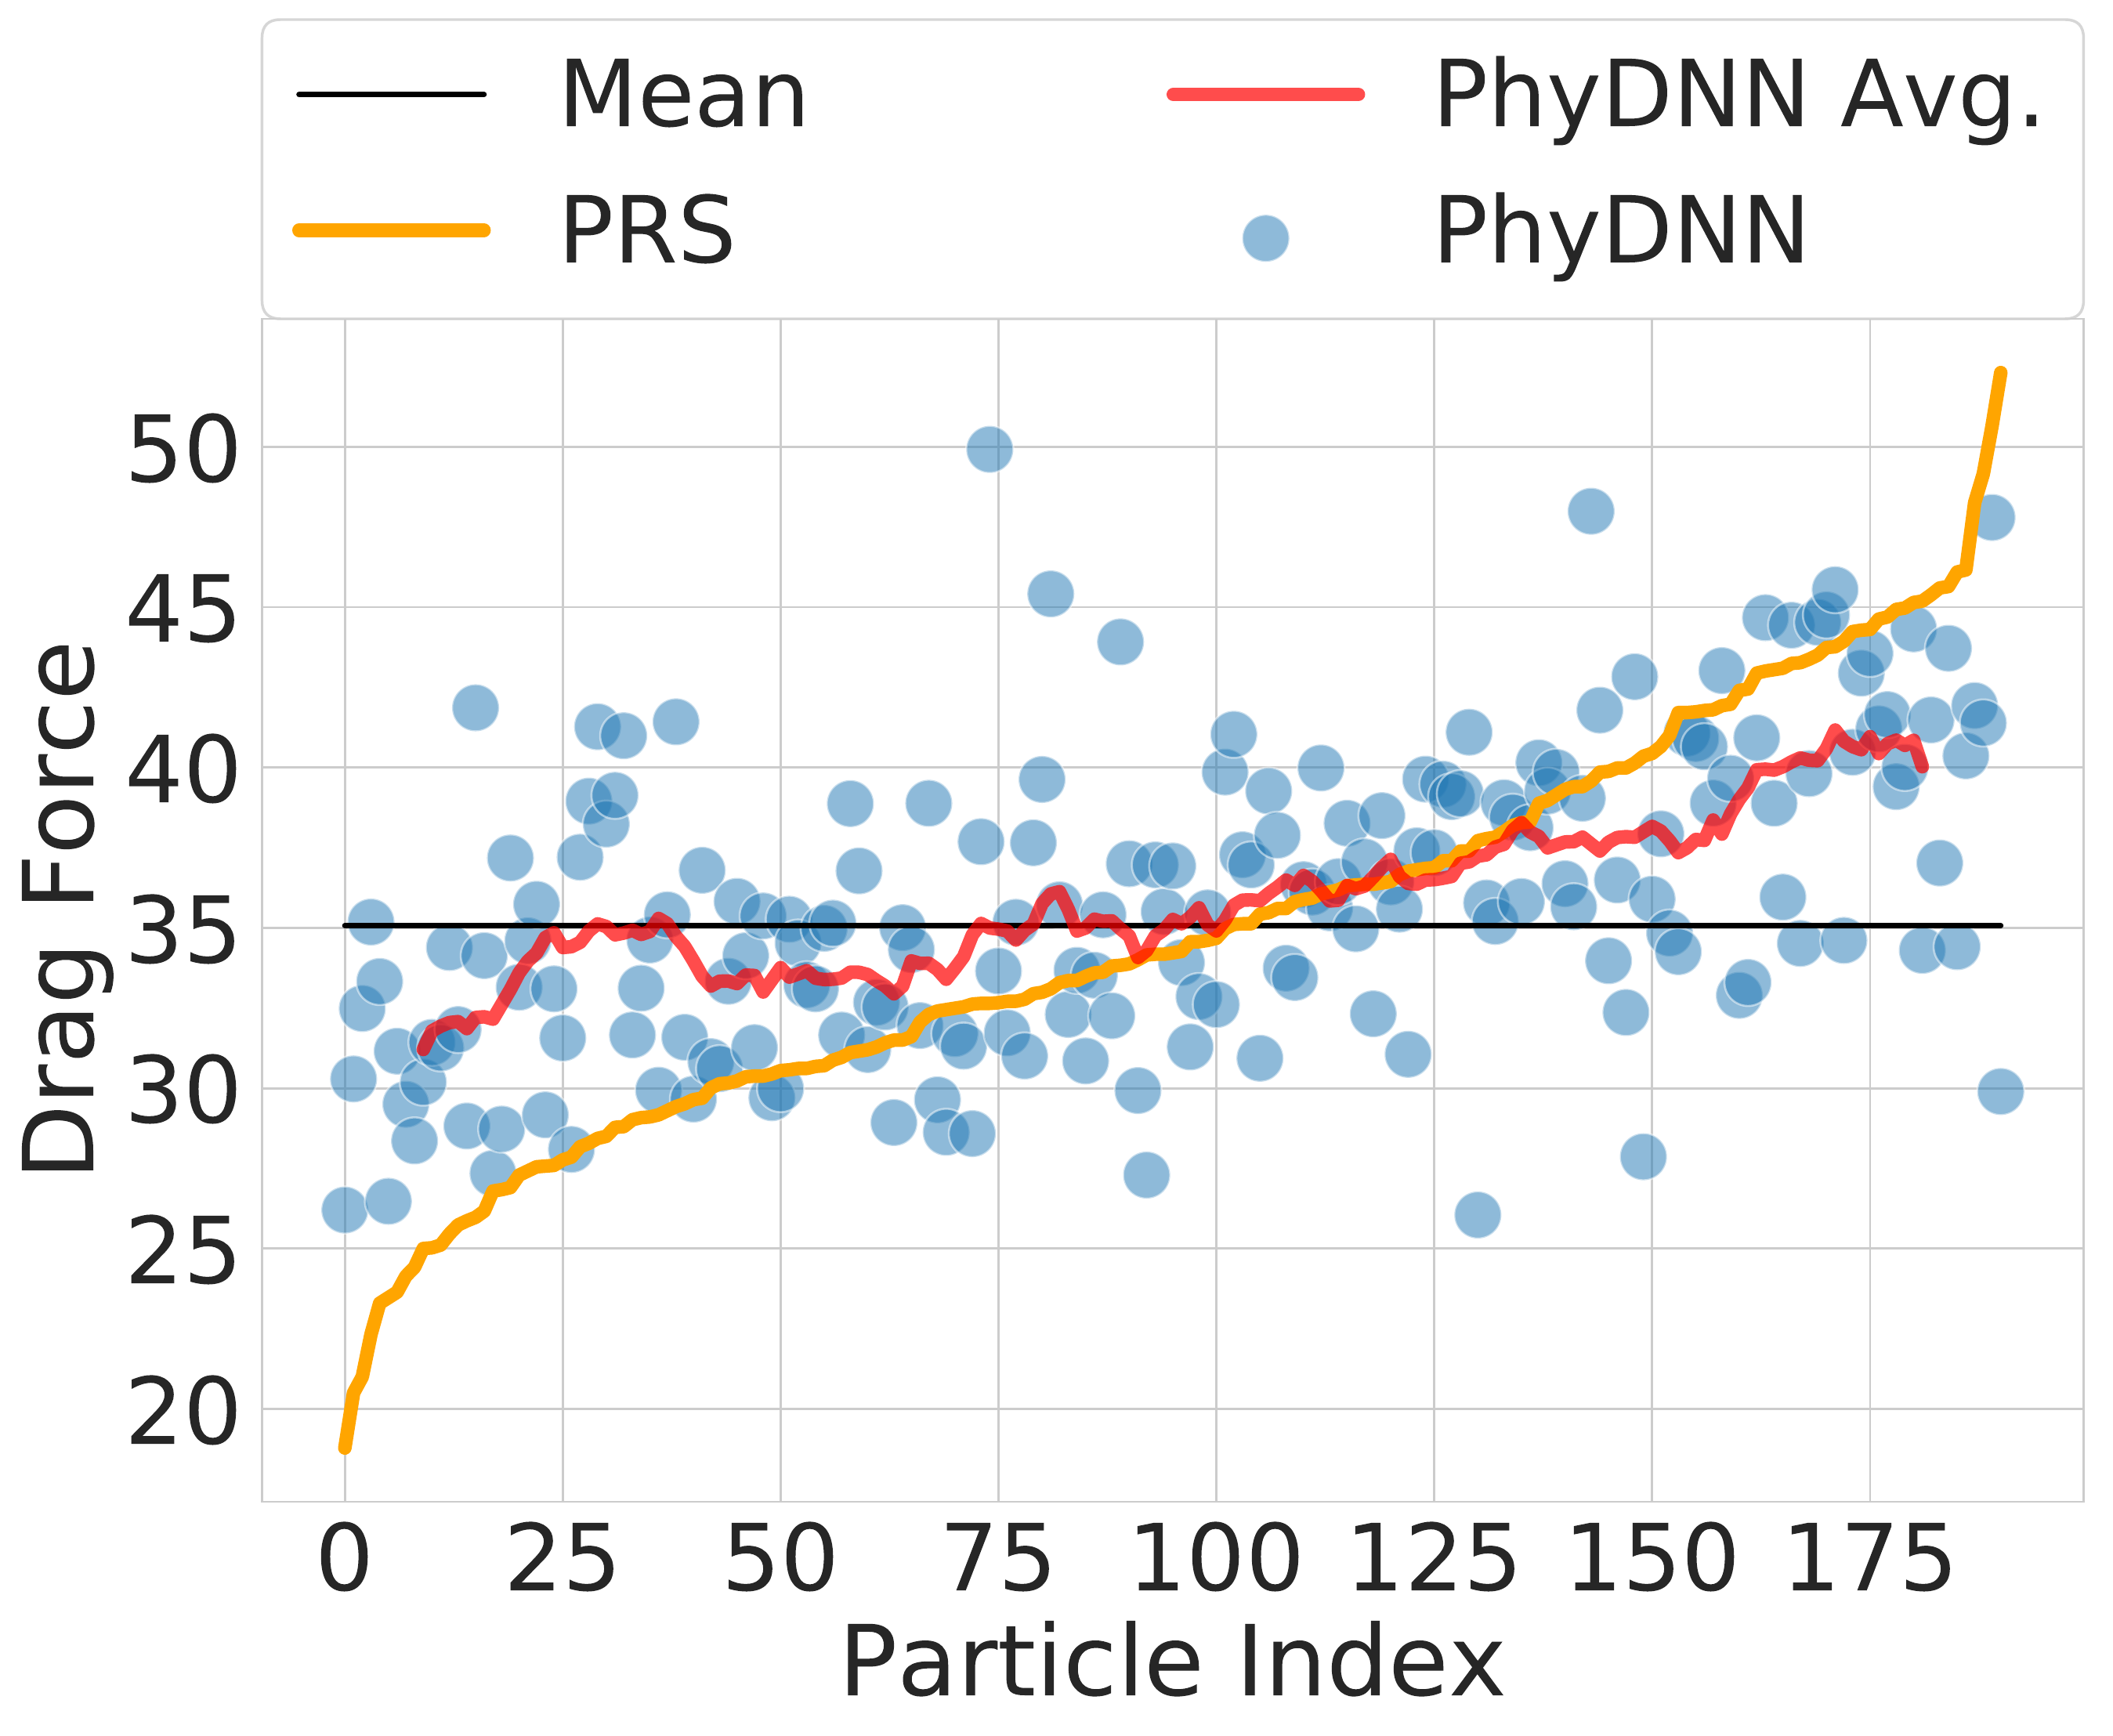}
         \caption{$Re = 200, \phi = 0.3$}
         \label{fig:re_200_sf_30}
     \end{subfigure}
     \hfill
     \begin{subfigure}[b]{0.48\columnwidth}
         \centering
         \includegraphics[width=\textwidth]{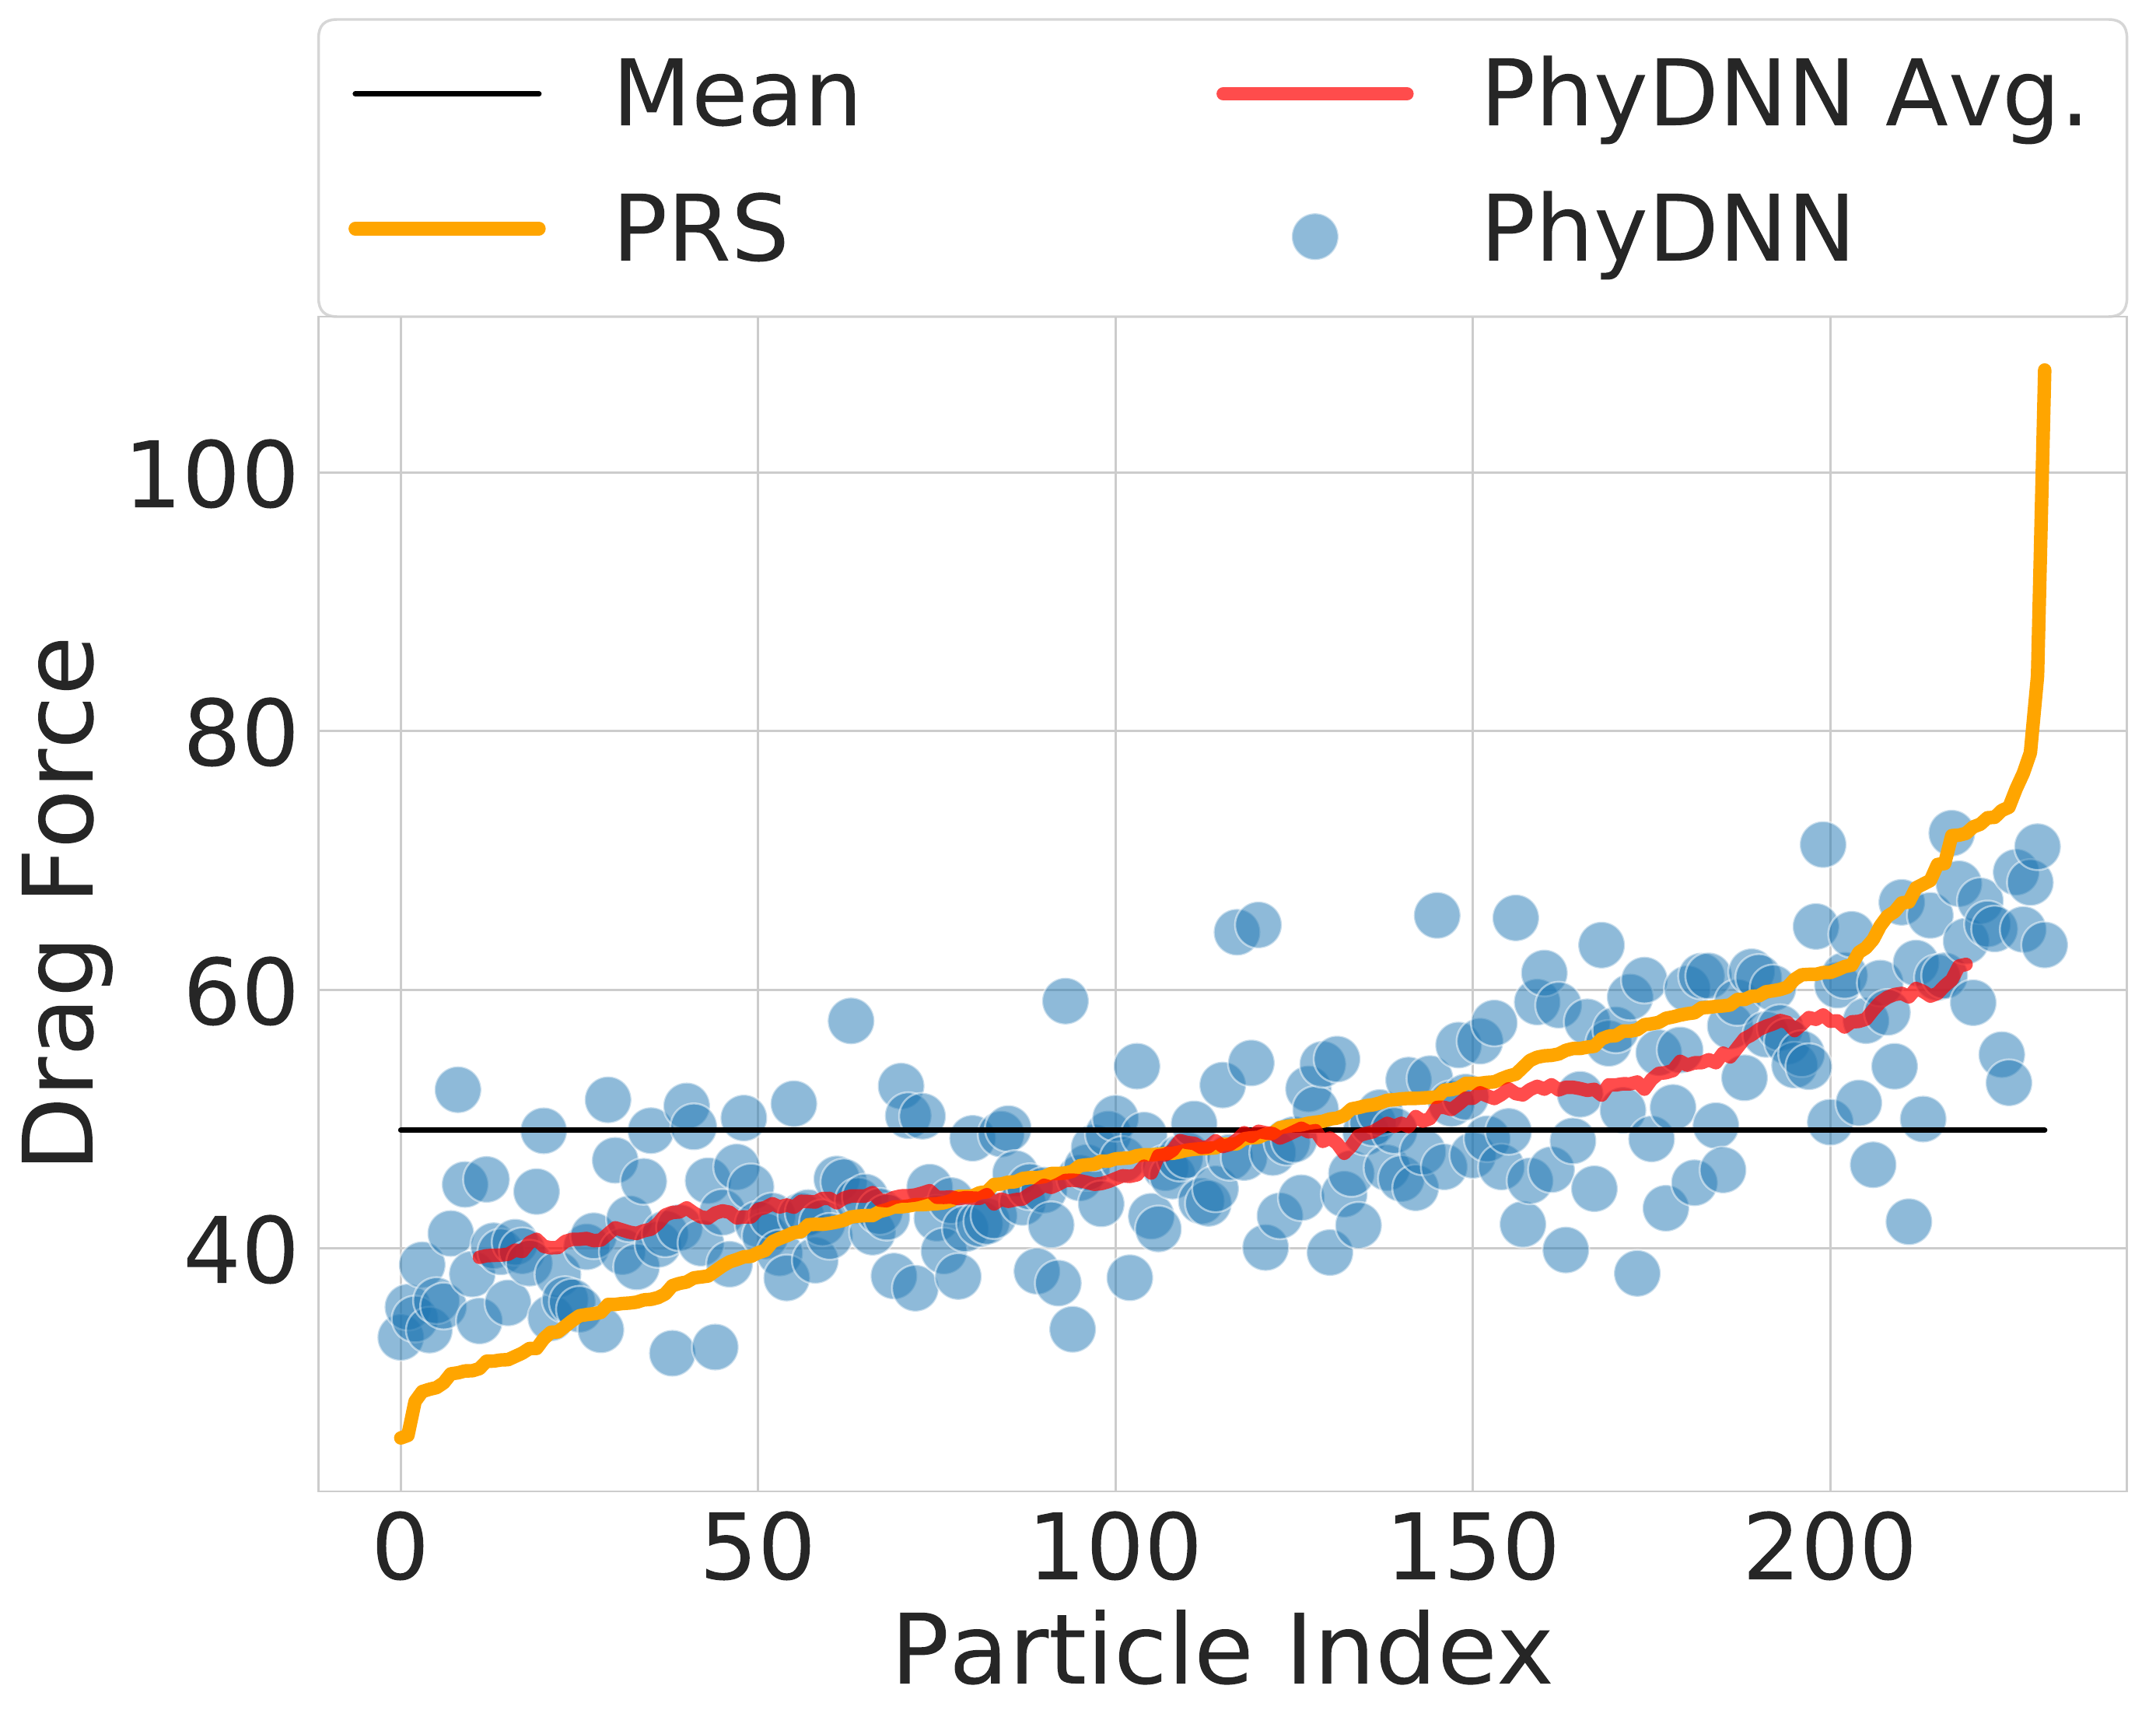}
         \caption{$Re = 200, \phi = 0.35$}
         \label{fig:re_200_sf_35}
     \end{subfigure}
        \caption{Each figure shows a comparison between \ourmethodAll predictions (red curve) and ground truth drag force data (yellow curve), for different (Re,$\phi$) cases..We also showcase the mean drag force value for each (Re,$\phi$) case (black). \iffalse The top row of figures indicates experiments conducted with low Re i.e Re=10 and different $\phi$ values. Notice that as $\phi$ increases, the number of samples is higher and hence the model is able to achieve a better representation of the corresponding PRS data curve (yellow).\fi  \iffalse We also notice that as Re and $\phi$ increase, the degree of non-linearity of the system increases due to the increase in complexity of the interactions between the particles. The magnitude of drag forces is also higher at higher Re and $\phi$ values.\fi}
        \label{fig:prs_scatter_plots}
\end{figure*}

\subsection{Hyperparameter Sensitivity}
Each of the four auxiliary tasks in the \ourmethod models, is governed by a hyperparameter during model training (refer to Section 3 in the main paper). In our experiments, we only tune the hyperparameters for the pressure field and velocity field prediction tasks leaving all other hyperparameters set to static values for all experiments. We employ a grid search procedure on the validation set to select the optimal hyperparameter values for the pressure and velocity field prediction auxiliary tasks in the \ourmethodAll model. In order to characterize the effect of this hyperparameter selection procedure on the model evaluation, we evaluate the sensitivity of the model to different hyperparameter values. 
\begin{figure}[!ht]
    \centering
    \includegraphics[scale=0.2]{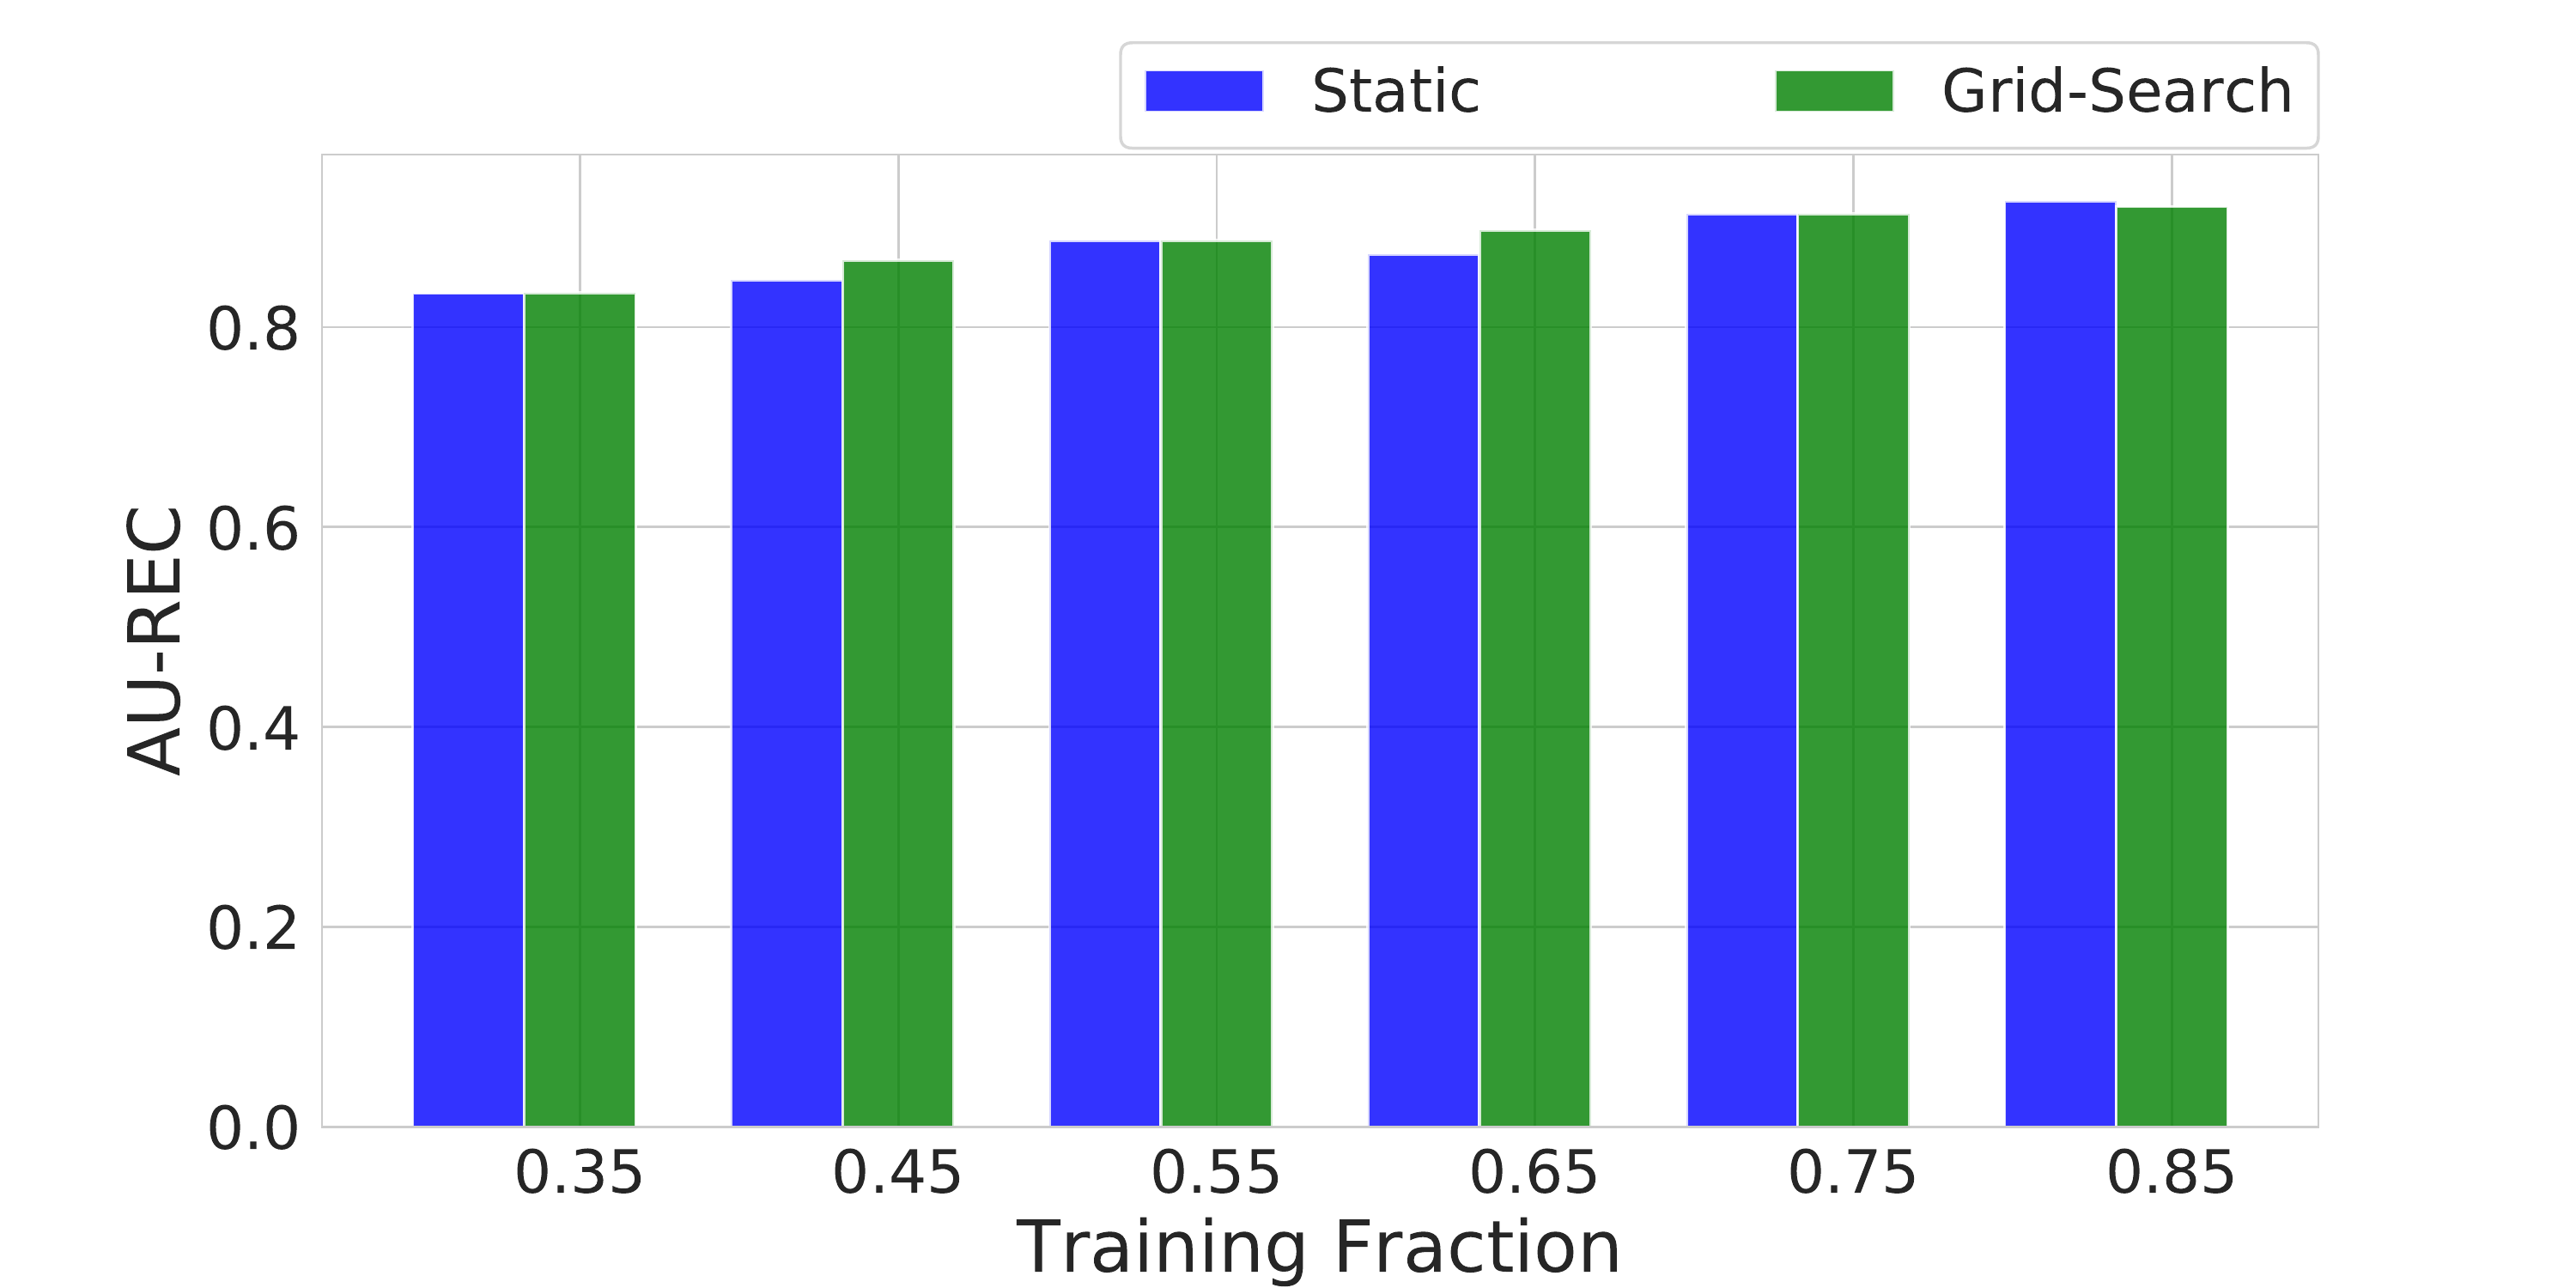}
    \caption{Hyperparameter sensitivity evaluation of the grid search hyperparameter selection procedure for the \ourmethodAll model. We notice that \ourmethodAll is robust to different settings of hyperparameters as we do not see significant changes in the AU-REC between the settings where hyperparameters for the \ourmethodAll were selected through grid search on the validation set (green) and the settings wherein the hyperparameter values were set by hand before the experiment (blue).}
    \label{fig:parameter_sensitivity_phydnnall}
\end{figure}
\begin{table}[!t]
    \centering
    \begin{tabular}{|c|c|c|}
        \hline
         Training Fraction& $\lambda_P$
         &$\lambda_V$\\ \hline
         0.35& $1e^{-2}$& $1e^{-1}$\\ \hline
         0.45& $1e^{-4}$&$1e^{-1}$\\ \hline
         0.55& $1e^{-4}$&$1e^{-3}$\\ \hline
         0.65& $1e^{-4}$&$1e^{-1}$\\ \hline
         0.75& $1e^{-2}$&$1e^{-3}$\\ \hline
         0.85& $1e^{-4}$&$1e^{-2}$\\ \hline

    \end{tabular}
    \caption{The table showcases hyperparameter values of \ourmethodAll, for different levels of training fractions each obtained through gridsearch. It must be noted that only the hyperparameters for the pressure and velocity field prediction auxiliary tasks were tuned and the rest of the values were kept constant for all experiments {$\lambda_{FP}=0.01, \lambda_{FS}=0.01$}.}
    \label{tab:hyperparameter_values}
\end{table}
\par\noindent We design the hyperparameter sensitivity experiment to inspect how model performance varies with different training fractions (i.e different experimental settings). We conduct an experiment by reducing the training fraction from 0.85 (85\% of data used for training) to 0.35 (35\% data used for training). Fig.~\ref{fig:parameter_sensitivity_phydnnall} shows the results of our experiment wherein the blue bars indicate the AU-REC values obtained when the \ourmethodAll model was trained with a static (predefined) set of hyperparameters\footnote{The optimal hyperparameters for the 0.55 training fraction case were used for all other settings.}. The green bars indicate the setting where the optimal hyperparameters for pressure and velocity field prediction for the \ourmethodAll model were obtained through gridsearch on the validation set. We notice that over all the training fractions, there is no significant difference between the two models and hence conclude that the \ourmethodAll model is robust across different hyperparameter settings. Exact hyperparameter values are detailed in Table.~\ref{tab:hyperparameter_values}.
